# Supplementary material for: Superstructure Optimization with Embedded Neural Networks for Sustainable Aviation Fuel Production
Source: arXiv:2509.09796 source file (2025-12-03)
Supplement: Supplementary file 1 [file SI.pdf]

# Electronic Supplementary Information. Superstructure Optimization with Embedded Neural Networks for Sustainable Aviation Fuel Production.

Alexander Klimek,<sup>a</sup> Christoph Plate,<sup>bc</sup> Sebastian Sager,<sup>bc</sup> Kai Sundmacher<sup>ad</sup> and  
Caroline Ganzer<sup>\*a</sup>

<sup>a</sup> Max Planck Institute for Dynamics of Complex Technical Systems, Department of Process Systems  
Engineering, Sandtorstr. 1, 39106 Magdeburg, Germany.

<sup>b</sup> Max Planck Institute for Dynamics of Complex Technical Systems, Mathematical Optimization and  
Machine Learning Group, Sandtorstr. 1, 39106 Magdeburg, Germany.

<sup>c</sup> Otto von Guericke University, Chair of Mathematical Algorithmic Optimization, Universitätsplatz 2,  
39106 Magdeburg, Germany.

<sup>d</sup> Otto von Guericke University, Chair for Process Systems Engineering, Universitätsplatz 2, 39106  
Magdeburg, Germany.

\*corresponding author; E-mail: cganzer@mpi-magdeburg.mpg.de

# A. Data

## A.1. Nomenclature

### Greek symbols

|            | description                                                | unit                                                                        |
|------------|------------------------------------------------------------|-----------------------------------------------------------------------------|
| $\alpha$   | chain growth probability                                   | – or %                                                                      |
| $\beta$    | specific CAPEX                                             | \$/capacity                                                                 |
| $\Gamma$   | process scale                                              | kg/h                                                                        |
| $\gamma$   | specific OPEX                                              | \$/kg or \$/kWh                                                             |
| $\Delta T$ | temperature difference                                     | K or °C                                                                     |
| $\delta$   | specific energy                                            | MJ/kg                                                                       |
| $\epsilon$ | binary variable for the activation status of an ANN neuron | –                                                                           |
| $\theta$   | project lifetime                                           | years                                                                       |
| $\lambda$  | specific CO <sub>2</sub> -equivalent emission intensities  | kg <sub>CO<sub>2</sub>-eq</sub> /kg or kg <sub>CO<sub>2</sub>-eq</sub> /kWh |
| $\nu$      | specific consumption/production                            | kg/h/reference capacity                                                     |
| $\sigma$   | activation function of an ANN                              | –                                                                           |
| $\tau$     | annual plant operating time                                | h                                                                           |

### Latin symbols

|      | description             | unit |
|------|-------------------------|------|
| $b$  | bias vector of an ANN   | –    |
| $CF$ | correction factor       | –    |
| $CR$ | capital recovery factor | –    |

|           | description                                                                            | unit                  |
|-----------|----------------------------------------------------------------------------------------|-----------------------|
| $e$       | specific work/electricity generation/consumption                                       | kW/reference capacity |
| $f$       | function                                                                               | —                     |
| $K$       | cost                                                                                   | \$                    |
| $k$       | specific cost                                                                          | \$/kg                 |
| $\dot{M}$ | mass flow                                                                              | kg/h                  |
| $n$       | number of carbon atoms                                                                 | —                     |
| $p$       | pressure                                                                               | bar                   |
| $\dot{Q}$ | thermal duty                                                                           | kW                    |
| $q$       | specific heat generation/consumption                                                   | kW/reference capacity |
| $r$       | interest rate                                                                          | — or %                |
| $S$       | selectivity                                                                            | — or %                |
| $T$       | temperature                                                                            | K                     |
| $W$       | weight matrix of an ANN                                                                | —                     |
| $\dot{W}$ | work/electricity flow                                                                  | kW                    |
| $w$       | mass fraction                                                                          | —                     |
| $x$       | binary variable for the selection of a biomass type/mole fraction/vector of ANN inputs | —                     |
| $y$       | binary variable for the decision whether to install a process or not                   | —                     |
| $z$       | binary variable that indicates whether a heat exchange link is active or not           | —                     |

## Sets

|                                 | description                                         |
|---------------------------------|-----------------------------------------------------|
| $\mathcal{C}$                   | set of components                                   |
| $\mathcal{C}^{\text{biomass}}$  | set of different biomass types                      |
| $\mathcal{C}^{\text{diesel}}$   | set of hydrocarbons considered as diesel fraction   |
| $\mathcal{C}^{\text{gasoline}}$ | set of hydrocarbons considered as gasoline fraction |
| $\mathcal{C}^{\text{HC}}$       | set of hydrocarbons considered as FT output         |

|                                  | description                                                        |
|----------------------------------|--------------------------------------------------------------------|
| $\mathcal{C}^K$                  | set of key reaction components                                     |
| $\mathcal{C}^{\text{kerosene}}$  | set of hydrocarbons considered as kerosene fraction                |
| $\mathcal{C}^{\text{src}}$       | set of source components                                           |
| $\mathcal{H}$                    | set of possible process heat sources/sinks                         |
| $\mathcal{I}$                    | set of possible process inlet ports                                |
| $\mathcal{J}$                    | set of processes                                                   |
| $\mathcal{J}^{\text{ANN}}$       | set of processes represented via an artificial neural network      |
| $\mathcal{J}^{\text{heat}}$      | set of suitable processes for heat integration                     |
| $\mathcal{J}^{\text{heat,cold}}$ | set of process heat sinks for heat integration                     |
| $\mathcal{J}^{\text{heat,hot}}$  | set of process heat sources for heat integration                   |
| $\mathcal{J}^{\text{heat,s}}$    | set of process heat sources/sinks for heat integration             |
| $\mathcal{J}^{\text{I}}$         | set of existing process inlet ports                                |
| $\mathcal{J}^{\text{O}}$         | set of existing process outlet ports                               |
| $\mathcal{J}^{\text{OI}}$        | set of existing connections between process outlet and inlet ports |
| $\mathcal{O}$                    | set of possible process outlet ports                               |

## Superscript and subscript indices

|          | description                                                    |
|----------|----------------------------------------------------------------|
| $\alpha$ | index for components                                           |
| $h$      | index for heat sources/sinks                                   |
| $i$      | index for process inlet ports/neurons within an ANN/ANN inputs |
| $j$      | index for processes                                            |
| $l$      | index for ANN layers                                           |
| $n$      | index for number of carbon atoms                               |
| $o$      | index for process outlet ports/ANN outputs                     |
| ANN      | artificial neural network                                      |
| ab       | abatement                                                      |
| cap      | CAPEX                                                          |
| comp     | component                                                      |
| el       | electricity                                                    |
| elec     | electrolysis                                                   |

|          | description  |
|----------|--------------|
| eq       | equivalent   |
| flow     | flow         |
| gas      | gasification |
| HC       | hydrocarbon  |
| in       | inlet        |
| kerosene | kerosene     |
| op       | OPEX         |
| out      | outlet       |
| ref      | reforming    |
| sq       | sequestered  |
| src      | source       |
| tot      | total        |

## Acronyms and abbreviations

|           | description                                |
|-----------|--------------------------------------------|
| AEC       | alkaline electrolysis cells                |
| AGR       | acid gas removal                           |
| ANN       | artificial neural network                  |
| API       | application programming interface          |
| ASF       | Anderson-Schulz-Flory                      |
| ASTM      | American Society for Testing and Materials |
| ASU       | air separation unit                        |
| ATJ       | alcohol-to-jet                             |
| ATR       | autothermal reforming                      |
| CAPEX     | capital expenditure                        |
| CRD       | cryogenic distillation                     |
| CS        | carbon sequestration                       |
| DAC       | direct air capture                         |
| FC        | fixed carbon                               |
| FT        | Fischer-Tropsch                            |
| GHG       | greenhouse gas                             |
| HEFA      | hydroprocessed esters and fatty acids      |
| heat int. | heat integration                           |

|       | description                                         |
|-------|-----------------------------------------------------|
| LB    | lower bound                                         |
| LHS   | latin hypercube sampling                            |
| MAE   | mean absolute error                                 |
| MAPE  | mean absolute percentage error                      |
| MILP  | mixed-integer linear programming                    |
| MINLP | mixed-integer nonlinear programming                 |
| MIQCP | mixed-integer quadratically constrained programming |
| MIS   | miscanthus                                          |
| MSE   | mean squared error                                  |
| MtJ   | methanol-to-jet                                     |
| MtO   | methanol-to-olefins                                 |
| OMLT  | Optimization & Machine Learning Toolkit             |
| OPEX  | operating expenditure                               |
| PC    | pine chips                                          |
| PEMEC | proton exchange membrane electrolysis cells         |
| PR-BM | Peng-Robinson-Boston-Mathias                        |
| PS    | point source                                        |
| ReLU  | rectified linear unit                               |
| RWGS  | reverse water-gas shift                             |
| ref.  | reference                                           |
| SAF   | sustainable aviation fuel                           |
| SMR   | steam methane reforming                             |
| SOEC  | solid oxide electrolysis cells                      |
| SPK   | synthetic paraffinic kerosene                       |
| UB    | upper bound                                         |
| VM    | volatile matter                                     |
| WS    | wheat straw                                         |
| wt.   | weight                                              |

## A.2. Set defintions

Set of all components of the system:

$$\mathcal{C} = \{\text{H}_2\text{O}, \text{H}_2\text{O}_{\text{waste}}, \text{Air}, \text{CO}_{2,\text{air}}, \text{CO}_2, \text{Miscanthus}, \text{WheatStraw}, \text{PineChips}, \\ \text{SolidWaste}, \text{H}_2, \text{O}_2, \text{N}_2, \text{CO}, \text{H}_2\text{S}, \text{HCl}, \text{NH}_3, \text{CH}_4, \text{C}_2\text{H}_6, \text{C}_3\text{H}_8, \text{C}_4\text{H}_{10}, \\ \text{C}_5\text{H}_{12}, \text{C}_6\text{H}_{14}, \text{C}_7\text{H}_{16}, \text{C}_8\text{H}_{18}, \text{C}_9\text{H}_{20}, \text{C}_{10}\text{H}_{22}, \text{C}_{11}\text{H}_{24}, \text{C}_{12}\text{H}_{26}, \text{C}_{13}\text{H}_{28}, \text{C}_{14}\text{H}_{30}, \\ \text{C}_{15}\text{H}_{32}, \text{C}_{16}\text{H}_{34}, \text{C}_{17}\text{H}_{36}, \text{C}_{18}\text{H}_{38}, \text{C}_{19}\text{H}_{40}, \text{C}_{20}\text{H}_{42}, \text{C}_{21}\text{H}_{44}, \text{C}_{22}\text{H}_{46}, \text{C}_{23}\text{H}_{48}, \\ \text{C}_{24}\text{H}_{50}, \text{C}_{25}\text{H}_{52}, \text{C}_{26}\text{H}_{54}, \text{C}_{27}\text{H}_{56}, \text{C}_{28}\text{H}_{58}, \text{C}_{29}\text{H}_{60}, \text{C}_{30}\text{H}_{62}, \text{C}_{30+}\}.$$

Set of all source components of the system:

$$\mathcal{C}^{\text{src}} = \{\text{H}_2\text{O}, \text{Air}, \text{CO}_{2,\text{air}}, \text{CO}_2, \text{Miscanthus}, \text{WheatStraw}, \text{PineChips}, \text{CH}_4\} \subseteq \mathcal{C}.$$

Set of different biomass types of the system:

$$\mathcal{C}^{\text{biomass}} = \{\text{Miscanthus}, \text{WheatStraw}, \text{PineChips}\} \subseteq \mathcal{C}.$$

Set of all hydrocarbons (n-alkanes) considered as FT output:

$$\mathcal{C}^{\text{HC}} = \{\text{CH}_4, \text{C}_2\text{H}_6, \text{C}_3\text{H}_8, \text{C}_4\text{H}_{10}, \text{C}_5\text{H}_{12}, \text{C}_6\text{H}_{14}, \text{C}_7\text{H}_{16}, \text{C}_8\text{H}_{18}, \text{C}_9\text{H}_{20}, \text{C}_{10}\text{H}_{22}, \\ \text{C}_{11}\text{H}_{24}, \text{C}_{12}\text{H}_{26}, \text{C}_{13}\text{H}_{28}, \text{C}_{14}\text{H}_{30}, \text{C}_{15}\text{H}_{32}, \text{C}_{16}\text{H}_{34}, \text{C}_{17}\text{H}_{36}, \text{C}_{18}\text{H}_{38}, \text{C}_{19}\text{H}_{40}, \\ \text{C}_{20}\text{H}_{42}, \text{C}_{21}\text{H}_{44}, \text{C}_{22}\text{H}_{46}, \text{C}_{23}\text{H}_{48}, \text{C}_{24}\text{H}_{50}, \text{C}_{25}\text{H}_{52}, \text{C}_{26}\text{H}_{54}, \text{C}_{27}\text{H}_{56}, \text{C}_{28}\text{H}_{58}, \\ \text{C}_{29}\text{H}_{60}, \text{C}_{30}\text{H}_{62}, \text{C}_{30+}\} \subseteq \mathcal{C}.$$

Set of all hydrocarbons (n-alkanes) considered as gasoline fraction:

$$\mathcal{C}^{\text{gasoline}} = \{\text{C}_1\text{H}_4, \text{C}_2\text{H}_6, \text{C}_3\text{H}_8, \text{C}_4\text{H}_{10}, \text{C}_5\text{H}_{12}, \text{C}_6\text{H}_{14}, \text{C}_7\text{H}_{16}\} \subseteq \mathcal{C}.$$

Set of all hydrocarbons (n-alkanes) considered as kerosene fraction:

$$\mathcal{C}^{\text{kerosene}} = \{\text{C}_8\text{H}_{18}, \text{C}_9\text{H}_{20}, \text{C}_{10}\text{H}_{22}, \text{C}_{11}\text{H}_{24}, \text{C}_{12}\text{H}_{26}, \text{C}_{13}\text{H}_{28}, \text{C}_{14}\text{H}_{30}, \text{C}_{15}\text{H}_{32}, \\ \text{C}_{16}\text{H}_{34}\} \subseteq \mathcal{C}.$$

Set of all hydrocarbons (n-alkanes) considered as diesel fraction:

$$\mathcal{C}^{\text{diesel}} = \{\text{C}_{17}\text{H}_{36}, \text{C}_{18}\text{H}_{38}, \text{C}_{19}\text{H}_{40}, \text{C}_{20}\text{H}_{42}, \text{C}_{21}\text{H}_{44}, \text{C}_{22}\text{H}_{46}, \text{C}_{23}\text{H}_{48}, \text{C}_{24}\text{H}_{50}, \\ \text{C}_{25}\text{H}_{52}, \text{C}_{26}\text{H}_{54}, \text{C}_{27}\text{H}_{56}, \text{C}_{28}\text{H}_{58}, \text{C}_{29}\text{H}_{60}, \text{C}_{30}\text{H}_{62}, \text{C}_{30+}\} \subseteq \mathcal{C}.$$

Set of all processes of the system:

$$\mathcal{J} = \{\text{DAC}, \text{CS}, \text{CRD}, \text{Gasification}, \text{ATR}, \text{AEC}, \text{PEMEC}, \text{SOEC}, \text{RWGS}, \text{AGR}, \text{FT}\}.$$

Set of all processes of the system represented via an artificial neural network (ANN):

$$\mathcal{J}^{\text{ANN}} = \{\text{Gasification}, \text{RWGS}, \text{FT}\} \subseteq \mathcal{J}.$$

Set of possible inlet ports of the processes of the system:

$$\mathcal{I} = \{1, 2, 3, 4, 5\}.$$

Set of possible outlet ports of the processes of the system:

$$\mathcal{O} = \{1, 2, 3\}.$$

Set of all existing process inlet ports of the system:

$$\begin{aligned} \mathcal{J}^I = \{ & (\text{DAC}, 1), (\text{CS}, 1), (\text{CRD}, 1), (\text{Gasification}, 1), (\text{Gasification}, 2), \\ & (\text{Gasification}, 3), (\text{Gasification}, 4), (\text{Gasification}, 5), (\text{ATR}, 1), (\text{AEC}, 1), \\ & (\text{PEMEC}, 1), (\text{SOEC}, 1), (\text{RWGS}, 1), (\text{AGR}, 1), (\text{FT}, 1) \} \subseteq \mathcal{J} \times \mathcal{I}. \end{aligned}$$

Set of all existing process outlet ports of the system:

$$\begin{aligned} \mathcal{J}^O = \{ & (\text{DAC}, 1), (\text{CS}, 1), (\text{CRD}, 1), (\text{CRD}, 2), (\text{Gasification}, 1), (\text{Gasification}, 2), \\ & (\text{Gasification}, 3), (\text{ATR}, 1), (\text{ATR}, 2), (\text{AEC}, 1), (\text{AEC}, 2), (\text{PEMEC}, 1), \\ & (\text{PEMEC}, 2), (\text{SOEC}, 1), (\text{SOEC}, 2), (\text{RWGS}, 1), (\text{RWGS}, 2), (\text{AGR}, 1), \\ & (\text{AGR}, 2), (\text{AGR}, 3), (\text{FT}, 1), (\text{FT}, 2), (\text{FT}, 3) \} \subseteq \mathcal{J} \times \mathcal{O}. \end{aligned}$$

Set of all existing connections between process outlet and inlet ports:

$$\begin{aligned} \mathcal{J}^{OI} = \{ & (\text{DAC}, 1, \text{CS}, 1), (\text{DAC}, 1, \text{Gasification}, 3), (\text{DAC}, 1, \text{RWGS}, 1), \\ & (\text{CRD}, 2, \text{Gasification}, 4), (\text{CRD}, 2, \text{ATR}, 1), (\text{Gasification}, 1, \text{AGR}, 1), \\ & (\text{ATR}, 1, \text{AGR}, 1), (\text{ATR}, 2, \text{RWGS}, 1), (\text{AEC}, 1, \text{RWGS}, 1), (\text{AEC}, 1, \text{FT}, 1), \\ & (\text{AEC}, 2, \text{Gasification}, 4), (\text{AEC}, 2, \text{ATR}, 1), (\text{PEMEC}, 1, \text{RWGS}, 1), \\ & (\text{PEMEC}, 1, \text{FT}, 1), (\text{PEMEC}, 2, \text{Gasification}, 4), (\text{PEMEC}, 2, \text{ATR}, 1), \\ & (\text{SOEC}, 1, \text{RWGS}, 1), (\text{SOEC}, 1, \text{FT}, 1), (\text{SOEC}, 2, \text{Gasification}, 4), \\ & (\text{SOEC}, 2, \text{ATR}, 1), (\text{RWGS}, 1, \text{AGR}, 1), (\text{AGR}, 1, \text{FT}, 1), \\ & (\text{AGR}, 2, \text{CS}, 1) \} \subseteq \mathcal{J}^O \times \mathcal{J}^I. \end{aligned}$$

Set of key reaction components of processes that are not represented via an ANN:

$$\mathcal{C}^K = \{(\text{CO}_2, \text{DAC}), (\text{CO}_2, \text{CS}), (\text{N}_2, \text{CRD}), (\text{H}_2, \text{ATR}), (\text{H}_2, \text{AEC}), (\text{H}_2, \text{PEMEC}), (\text{H}_2, \text{SOEC}), (\text{CO}_2, \text{AGR})\} \subseteq \mathcal{C} \times \mathcal{J}.$$

Set of possible heat sources/sinks of the processes considered for possible heat integration:

$$\mathcal{H} = \{1, 2, 3\}.$$

Set of all suitable processes for possible heat integration:

$$\mathcal{J}^{\text{heat}} = \{\text{DAC}, \text{Gasification}, \text{ATR}, \text{SOEC}, \text{RWGS}, \text{FT}\} \subseteq \mathcal{J}.$$

Set of all process heat sources/sinks considered for possible heat integration:

$$\mathcal{J}^{\text{heat,s}} = \{(\text{DAC}, 1), (\text{Gasification}, 1), (\text{Gasification}, 2), (\text{Gasification}, 3), (\text{ATR}, 1), (\text{SOEC}, 1), (\text{RWGS}, 1), (\text{RWGS}, 2), (\text{FT}, 1), (\text{FT}, 2)\} \subseteq \mathcal{J}^{\text{heat}} \times \mathcal{H}.$$

Set of all process heat sources considered for possible heat integration:

$$\mathcal{J}^{\text{heat,hot}} = \{(\text{Gasification}, 2), (\text{Gasification}, 3), (\text{ATR}, 1), (\text{RWGS}, 2), (\text{FT}, 1), (\text{FT}, 2)\} \subseteq \mathcal{J}^{\text{heat,s}}.$$

Set of all process heat sinks considered for possible heat integration:

$$\mathcal{J}^{\text{heat,cold}} = \{(\text{DAC}, 1), (\text{Gasification}, 1), (\text{Gasification}, 2), (\text{SOEC}, 1), (\text{RWGS}, 1)\} \subseteq \mathcal{J}^{\text{heat,s}}.$$

### A.3. Parameters

Table A.6.: Specific electricity generation/consumption  $e_j$  of processes  $j$  that are not represented via an ANN in kW/reference capacity.

| process $j$ | reference capacity                | $e_j$ / kW/reference capacity | ref. |
|-------------|-----------------------------------|-------------------------------|------|
| DAC         | 1 kg <sub>CO<sub>2</sub></sub> /h | -0.4                          | [1]  |
| CS          | 1 kg <sub>CO<sub>2</sub></sub> /h | -0.132                        | [2]  |
| CRD         | 1 kg <sub>N<sub>2</sub></sub> /h  | -0.12                         | [3]  |
| ATR         | 1 kg <sub>H<sub>2</sub></sub> /h  | -0.5413                       | [4]  |
| AEC         | 1 kg <sub>H<sub>2</sub></sub> /h  | -50                           | [3]  |
| PEMEC       | 1 kg <sub>H<sub>2</sub></sub> /h  | -45.42                        | [1]  |
| SOEC        | 1 kg <sub>H<sub>2</sub></sub> /h  | -34.65                        | [1]  |
| AGR         | 1 kg <sub>CO<sub>2</sub></sub> /h | -0.01964                      | [5]  |

Table A.7.: Specific heat generation/consumption  $q_{(j,h)}$  of process heat source/sink  $(j, h)$  where processes are not represented via an ANN in kW/reference capacity.

| process heat source/sink<br>$(j, h)$ | reference capacity                | $q_{(j,h)}$ /<br>kW/reference capacity | ref. |
|--------------------------------------|-----------------------------------|----------------------------------------|------|
| (DAC,1)                              | 1 kg <sub>CO<sub>2</sub></sub> /h | -2                                     | [1]  |
| (ATR,1)                              | 1 kg <sub>H<sub>2</sub></sub> /h  | 2.369                                  | [6]  |
| (SOEC,1)                             | 1 kg <sub>H<sub>2</sub></sub> /h  | -14                                    | [7]  |

Table A.8.: Temperature level  $T_{(j,h)}$  of process heat source/sink  $(j, h)$  where the temperature is not calculated via an ANN in °C.

| process heat source/sink $(j, h)$ | $T_{(j,h)} / ^\circ\text{C}$ | ref.   |
|-----------------------------------|------------------------------|--------|
| (DAC,1)                           | 100                          | [1]    |
| (ATR,1)                           | 900                          | [8, 9] |
| (SOEC,1)                          | 100*                         | [1]    |
| (Gasification,1)                  | 450                          | [10]   |
| (Gasification,3)                  | 300                          | [10]   |
| (RWGS,2)                          | 25                           | -      |
| (FT,2)                            | 60                           | -      |

\* It is assumed that most of the heat is required during the evaporation of the water. The remaining heat to keep the process at operating temperature is negligible [1].

Table A.9.: Specific consumption/production  $\nu_{\alpha,j}$  of component  $\alpha$  in process  $j$  where processes are not represented via an ANN in kg/h/reference capacity.

| component $\alpha$                | process $j$ / reference capacity  |                                   |                                  |                                  |                                  |                                  |                                  |                                   |
|-----------------------------------|-----------------------------------|-----------------------------------|----------------------------------|----------------------------------|----------------------------------|----------------------------------|----------------------------------|-----------------------------------|
|                                   | DAC                               | CS                                | CRD                              | ATR                              | AEC                              | PEMEC                            | SOEC                             | AGR                               |
|                                   | 1 kg <sub>CO<sub>2</sub></sub> /h | 1 kg <sub>CO<sub>2</sub></sub> /h | 1 kg <sub>N<sub>2</sub></sub> /h | 1 kg <sub>H<sub>2</sub></sub> /h | 1 kg <sub>H<sub>2</sub></sub> /h | 1 kg <sub>H<sub>2</sub></sub> /h | 1 kg <sub>H<sub>2</sub></sub> /h | 1 kg <sub>CO<sub>2</sub></sub> /h |
| H <sub>2</sub> O                  | 0                                 | 0                                 | 0                                | -2.393                           | -9                               | -9                               | -9                               | 0                                 |
| H <sub>2</sub> O <sub>waste</sub> | 0                                 | 0                                 | 0                                | 2.798                            | 0                                | 0                                | 0                                | 0                                 |
| Air                               | 0                                 | 0                                 | -1.31                            | 0                                | 0                                | 0                                | 0                                | 0                                 |
| CO <sub>2,air</sub>               | -1                                | 0                                 | 0                                | 0                                | 0                                | 0                                | 0                                | 0                                 |
| CO <sub>2</sub>                   | 1                                 | 0                                 | 0                                | 0.029                            | 0                                | 0                                | 0                                | 0                                 |
| Miscanthus                        | 0                                 | 0                                 | 0                                | 0                                | 0                                | 0                                | 0                                | 0                                 |
| WheatStraw                        | 0                                 | 0                                 | 0                                | 0                                | 0                                | 0                                | 0                                | 0                                 |
| PineChips                         | 0                                 | 0                                 | 0                                | 0                                | 0                                | 0                                | 0                                | 0                                 |
| SolidWaste                        | 0                                 | 0                                 | 0                                | 0                                | 0                                | 0                                | 0                                | 0                                 |
| H <sub>2</sub>                    | 0                                 | 0                                 | 0                                | 1                                | 1                                | 1                                | 1                                | 0                                 |
| O <sub>2</sub>                    | 0                                 | 0                                 | 0.31                             | -4.256                           | 8                                | 8                                | 8                                | 0                                 |
| N <sub>2</sub>                    | 0                                 | 0                                 | 1                                | 0                                | 0                                | 0                                | 0                                | 0                                 |
| CO                                | 0                                 | 0                                 | 0                                | 6.364                            | 0                                | 0                                | 0                                | 0                                 |
| H <sub>2</sub> S                  | 0                                 | 0                                 | 0                                | 0                                | 0                                | 0                                | 0                                | 0                                 |
| HCl                               | 0                                 | 0                                 | 0                                | 0                                | 0                                | 0                                | 0                                | 0                                 |
| NH <sub>3</sub>                   | 0                                 | 0                                 | 0                                | 0                                | 0                                | 0                                | 0                                | 0                                 |
| CH <sub>4</sub>                   | 0                                 | 0                                 | 0                                | -3.542                           | 0                                | 0                                | 0                                | 0                                 |
| C <sub>2</sub> H <sub>6</sub>     | 0                                 | 0                                 | 0                                | 0                                | 0                                | 0                                | 0                                | 0                                 |
| C <sub>3</sub> H <sub>8</sub>     | 0                                 | 0                                 | 0                                | 0                                | 0                                | 0                                | 0                                | 0                                 |
| C <sub>4</sub> H <sub>10</sub>    | 0                                 | 0                                 | 0                                | 0                                | 0                                | 0                                | 0                                | 0                                 |
| C <sub>5</sub> H <sub>12</sub>    | 0                                 | 0                                 | 0                                | 0                                | 0                                | 0                                | 0                                | 0                                 |
| C <sub>6</sub> H <sub>14</sub>    | 0                                 | 0                                 | 0                                | 0                                | 0                                | 0                                | 0                                | 0                                 |
| C <sub>7</sub> H <sub>16</sub>    | 0                                 | 0                                 | 0                                | 0                                | 0                                | 0                                | 0                                | 0                                 |
| C <sub>8</sub> H <sub>18</sub>    | 0                                 | 0                                 | 0                                | 0                                | 0                                | 0                                | 0                                | 0                                 |
| C <sub>9</sub> H <sub>20</sub>    | 0                                 | 0                                 | 0                                | 0                                | 0                                | 0                                | 0                                | 0                                 |
| C <sub>10</sub> H <sub>22</sub>   | 0                                 | 0                                 | 0                                | 0                                | 0                                | 0                                | 0                                | 0                                 |
| C <sub>11</sub> H <sub>24</sub>   | 0                                 | 0                                 | 0                                | 0                                | 0                                | 0                                | 0                                | 0                                 |
| C <sub>12</sub> H <sub>26</sub>   | 0                                 | 0                                 | 0                                | 0                                | 0                                | 0                                | 0                                | 0                                 |
| C <sub>13</sub> H <sub>28</sub>   | 0                                 | 0                                 | 0                                | 0                                | 0                                | 0                                | 0                                | 0                                 |
| C <sub>14</sub> H <sub>30</sub>   | 0                                 | 0                                 | 0                                | 0                                | 0                                | 0                                | 0                                | 0                                 |
| C <sub>15</sub> H <sub>32</sub>   | 0                                 | 0                                 | 0                                | 0                                | 0                                | 0                                | 0                                | 0                                 |
| C <sub>16</sub> H <sub>34</sub>   | 0                                 | 0                                 | 0                                | 0                                | 0                                | 0                                | 0                                | 0                                 |
| C <sub>17</sub> H <sub>36</sub>   | 0                                 | 0                                 | 0                                | 0                                | 0                                | 0                                | 0                                | 0                                 |
| C <sub>18</sub> H <sub>38</sub>   | 0                                 | 0                                 | 0                                | 0                                | 0                                | 0                                | 0                                | 0                                 |
| C <sub>19</sub> H <sub>40</sub>   | 0                                 | 0                                 | 0                                | 0                                | 0                                | 0                                | 0                                | 0                                 |
| C <sub>20</sub> H <sub>42</sub>   | 0                                 | 0                                 | 0                                | 0                                | 0                                | 0                                | 0                                | 0                                 |
| C <sub>21</sub> H <sub>44</sub>   | 0                                 | 0                                 | 0                                | 0                                | 0                                | 0                                | 0                                | 0                                 |
| C <sub>22</sub> H <sub>46</sub>   | 0                                 | 0                                 | 0                                | 0                                | 0                                | 0                                | 0                                | 0                                 |
| C <sub>23</sub> H <sub>48</sub>   | 0                                 | 0                                 | 0                                | 0                                | 0                                | 0                                | 0                                | 0                                 |
| C <sub>24</sub> H <sub>50</sub>   | 0                                 | 0                                 | 0                                | 0                                | 0                                | 0                                | 0                                | 0                                 |
| C <sub>25</sub> H <sub>52</sub>   | 0                                 | 0                                 | 0                                | 0                                | 0                                | 0                                | 0                                | 0                                 |
| C <sub>26</sub> H <sub>54</sub>   | 0                                 | 0                                 | 0                                | 0                                | 0                                | 0                                | 0                                | 0                                 |
| C <sub>27</sub> H <sub>56</sub>   | 0                                 | 0                                 | 0                                | 0                                | 0                                | 0                                | 0                                | 0                                 |
| C <sub>28</sub> H <sub>58</sub>   | 0                                 | 0                                 | 0                                | 0                                | 0                                | 0                                | 0                                | 0                                 |
| C <sub>29</sub> H <sub>60</sub>   | 0                                 | 0                                 | 0                                | 0                                | 0                                | 0                                | 0                                | 0                                 |
| C <sub>30</sub> H <sub>62</sub>   | 0                                 | 0                                 | 0                                | 0                                | 0                                | 0                                | 0                                | 0                                 |
| C <sub>30+</sub>                  | 0                                 | 0                                 | 0                                | 0                                | 0                                | 0                                | 0                                | 0                                 |

Table A.10.: Specific CAPEX  $\beta_j$  of processes  $j$  that are not represented via an ANN (without AGR) in \$/reference capacity.

| process $j$ | reference capacity                | $\beta_j$ / \$/reference capacity | ref. |
|-------------|-----------------------------------|-----------------------------------|------|
| DAC         | 1 kg <sub>CO<sub>2</sub></sub> /h | 7,260                             | [11] |
| CS          | 1 kg <sub>CO<sub>2</sub></sub> /h | 490                               | [2]  |
| CRD         | 1 kg <sub>N<sub>2</sub></sub> /h  | 260                               | [12] |
| ATR         | 1 kg <sub>H<sub>2</sub></sub> /h  | 3,500                             | [2]  |
| AEC         | 1 kg <sub>H<sub>2</sub></sub> /h  | 67,260                            | [7]  |
| PEMEC       | 1 kg <sub>H<sub>2</sub></sub> /h  | 73,750                            | [12] |
| SOEC        | 1 kg <sub>H<sub>2</sub></sub> /h  | 273,600                           | [7]  |

Table A.11.: Specific OPEX  $\gamma_\alpha^{\text{src}}$  of source components/ressources  $\alpha$  in \$/kg.

| component $\alpha$  | $\gamma_\alpha^{\text{src}}$ / \$/kg | ref.     |
|---------------------|--------------------------------------|----------|
| H <sub>2</sub> O    | 0.0016                               | [7]      |
| Air                 | 0                                    | -        |
| CO <sub>2,air</sub> | 0                                    | -        |
| CO <sub>2</sub>     | 0.029                                | [7]      |
| Miscanthus          | 0.18*                                | [13, 14] |
| WheatStraw          | 0.1796*                              | [13, 14] |
| PineChips           | 0.1664*                              | [13, 14] |
| CH <sub>4</sub>     | 0.44                                 | [15]     |

\* Costs are calculated using an average biomass cost of 10 \$/GJ from Meys et al. [13] and average higher heating values of miscanthus, wheat straw and pine chips from Nebeská et al. [14].

Table A.12.: Specific CO<sub>2</sub> emissions  $\lambda_{\alpha}^{\text{comp}}$  of source components/resources  $\alpha$  in kgCO<sub>2</sub>-eq/kg.

| component $\alpha$  | $\lambda_{\alpha}^{\text{comp}}$ / kgCO <sub>2</sub> -eq/kg | ref.     |
|---------------------|-------------------------------------------------------------|----------|
| H <sub>2</sub> O    | 0                                                           | -        |
| Air                 | 0                                                           | -        |
| CO <sub>2,air</sub> | -1                                                          | -        |
| CO <sub>2</sub>     | 0.120                                                       | [7]      |
| Miscanthus          | -1.0545*                                                    | [16, 17] |
| WheatStraw          | -1.0169*                                                    | [16, 17] |
| PineChips           | -1.1855*                                                    | [16, 17] |
| CH <sub>4</sub>     | 0.39138                                                     | [18]     |

\* CO<sub>2</sub> uptakes of different biomass types are calculated based on data from Vassilev et al. [17] and average CO<sub>2</sub> supply chain emissions for biomass of 0.495 kgCO<sub>2</sub>/kg<sub>biomass</sub> from Cumicheo et al. [16] are added to these uptakes.

Table A.13.: Specific OPEX ( $\gamma$ ) and CO<sub>2</sub> emissions ( $\lambda$ ) of electricity and heat.

| parameter               | value / unit                    | ref. |
|-------------------------|---------------------------------|------|
| $\gamma^{\text{el}}$    | 0.1242 \$/kWh                   | [19] |
| $\gamma^{\text{heat}}$  | 0.0328 \$/kWh                   | [7]  |
| $\lambda^{\text{el}}$   | 0.36 kgCO <sub>2</sub> -eq/kWh  | [7]  |
| $\lambda^{\text{heat}}$ | 0.248 kgCO <sub>2</sub> -eq/kWh | [7]  |

Table A.14.: Physical properties (specific energy  $\delta_\alpha$  and specific CO<sub>2</sub> emissions  $\lambda_\alpha^{\text{comp}}$ ) of hydrocarbons (298.15 K) considered as FT output.

| component $\alpha$              | physical property / unit        |                                                              |
|---------------------------------|---------------------------------|--------------------------------------------------------------|
|                                 | $\delta_\alpha$ [20] /<br>MJ/kg | $\lambda_\alpha^{\text{comp}}$ /<br>kgCO <sub>2</sub> -eq/kg |
| CH <sub>4</sub>                 | 50.03004471                     | 2.7427                                                       |
| C <sub>2</sub> H <sub>6</sub>   | 47.51104436                     | 2.9265                                                       |
| C <sub>3</sub> H <sub>8</sub>   | 46.33268113                     | 2.9934                                                       |
| C <sub>4</sub> H <sub>10</sub>  | 45.71859182                     | 3.0280                                                       |
| C <sub>5</sub> H <sub>12</sub>  | 44.97473884                     | 3.0492                                                       |
| C <sub>6</sub> H <sub>14</sub>  | 44.73459093                     | 3.0635                                                       |
| C <sub>7</sub> H <sub>16</sub>  | 44.55638715                     | 3.0737                                                       |
| C <sub>8</sub> H <sub>18</sub>  | 44.42010972                     | 3.0815                                                       |
| C <sub>9</sub> H <sub>20</sub>  | 44.32128104                     | 3.0875                                                       |
| C <sub>10</sub> H <sub>22</sub> | 44.2368075                      | 3.092                                                        |
| C <sub>11</sub> H <sub>24</sub> | 44.16563944                     | 3.096                                                        |
| C <sub>12</sub> H <sub>26</sub> | 44.11030182                     | 3.1                                                          |
| C <sub>13</sub> H <sub>28</sub> | 44.05871994                     | 3.103                                                        |
| C <sub>14</sub> H <sub>30</sub> | 44.01796038                     | 3.105                                                        |
| C <sub>15</sub> H <sub>32</sub> | 43.98084202                     | 3.107                                                        |
| C <sub>16</sub> H <sub>34</sub> | 43.9462466                      | 3.109                                                        |
| C <sub>17</sub> H <sub>36</sub> | 43.92096837                     | 3.1105                                                       |
| C <sub>18</sub> H <sub>38</sub> | 43.89587426                     | 3.1120                                                       |
| C <sub>19</sub> H <sub>40</sub> | 43.87349335                     | 3.1133                                                       |
| C <sub>20</sub> H <sub>42</sub> | 43.85293715                     | 3.1145                                                       |
| C <sub>21</sub> H <sub>44</sub> | 43.69810597                     | 3.1155                                                       |
| C <sub>22</sub> H <sub>46</sub> | 43.6886146                      | 3.1165                                                       |
| C <sub>23</sub> H <sub>48</sub> | 43.64913953                     | 3.1174                                                       |
| C <sub>24</sub> H <sub>50</sub> | 43.67199057                     | 3.1182                                                       |
| C <sub>25</sub> H <sub>52</sub> | 43.63631662                     | 3.1189                                                       |
| C <sub>26</sub> H <sub>54</sub> | 43.63064088                     | 3.1200                                                       |
| C <sub>27</sub> H <sub>56</sub> | 43.59911881                     | 3.1202                                                       |
| C <sub>28</sub> H <sub>58</sub> | 43.62049943                     | 3.1208                                                       |
| C <sub>29</sub> H <sub>60</sub> | 43.59148855                     | 3.1214                                                       |
| C <sub>30</sub> H <sub>62</sub> | 43.58805312                     | 3.1219                                                       |
| C <sub>30+</sub>                | 43.5                            | 3.1220                                                       |

## B. Model formulation

### B.1. Process-specific constraints

In addition to the general constraints of the mixed-integer quadratically constrained programming (MIQCP) formulation, further process-specific constraints are introduced to ensure that only specified components are converted or generated in specific processes. The following subsections list all the process-specific constraints, whereby  $w$  describes the mass fraction of a component  $\alpha$  within a mass flow and  $y$  represents the binary decision variable for the installation of a process  $j$ . Thus, in the case of installing a process ( $y_j = 1$ ), the inlet and outlet mass fractions of the individual ports need to sum to one. If the corresponding process is not installed ( $y_j = 0$ ), the mass fractions are consequently set to zero.

#### B.1.1. Direct air capture (DAC)

$$w_{\text{CO}_2, \text{air}, (\text{DAC}, 1)}^{\text{in}} = y_{\text{DAC}} \quad (\text{B.1})$$

$$w_{\text{CO}_2, (\text{DAC}, 1)}^{\text{out}} = y_{\text{DAC}} \quad (\text{B.2})$$

#### B.1.2. Carbon sequestration (CS)

$$w_{\text{CO}_2, (\text{CS}, 1)}^{\text{in}} = y_{\text{CS}} \quad (\text{B.3})$$

$$w_{\text{CO}_2, (\text{CS}, 1)}^{\text{out}} = y_{\text{CS}} \quad (\text{B.4})$$

#### B.1.3. Cryogenic distillation (CRD)

$$w_{\text{Air}, (\text{CRD}, 1)}^{\text{in}} = y_{\text{CRD}} \quad (\text{B.5})$$

$$w_{\text{N}_2, (\text{CRD}, 1)}^{\text{out}} = y_{\text{CRD}} \quad (\text{B.6})$$

$$w_{\text{O}_2, (\text{CRD}, 2)}^{\text{out}} = y_{\text{CRD}} \quad (\text{B.7})$$

### B.1.4. Gasification

$$w_{\alpha,(\text{Gasification},1)}^{\text{in}} = x_{\alpha} \quad \forall \alpha \in \mathcal{C}^{\text{biomass}} \quad (\text{B.8})$$

$$\sum_{\alpha \in \mathcal{C}^{\text{biomass}}} x_{\alpha} = y_{\text{Gasification}} \quad (\text{B.9})$$

$$w_{\text{H}_2\text{O},(\text{Gasification},2)}^{\text{in}} = y_{\text{Gasification}} \quad (\text{B.10})$$

$$w_{\text{CO}_2,(\text{Gasification},3)}^{\text{in}} = y_{\text{Gasification}} \quad (\text{B.11})$$

$$w_{\text{O}_2,(\text{Gasification},4)}^{\text{in}} = y_{\text{Gasification}} \quad (\text{B.12})$$

$$w_{\text{H}_2\text{O},(\text{Gasification},5)}^{\text{in}} = y_{\text{Gasification}} \quad (\text{B.13})$$

$$\begin{aligned} w_{\text{H}_2,(\text{Gasification},1)}^{\text{out}} + w_{\text{CO},(\text{Gasification},1)}^{\text{out}} + w_{\text{CO}_2,(\text{Gasification},1)}^{\text{out}} + w_{\text{H}_2\text{O}_{\text{waste}},(\text{Gasification},1)}^{\text{out}} \\ + w_{\text{N}_2,(\text{Gasification},1)}^{\text{out}} + w_{\text{HCl},(\text{Gasification},1)}^{\text{out}} + w_{\text{H}_2\text{S},(\text{Gasification},1)}^{\text{out}} \\ + w_{\text{CH}_4,(\text{Gasification},1)}^{\text{out}} = y_{\text{Gasification}} \end{aligned} \quad (\text{B.14})$$

$$w_{\text{CO}_2,(\text{Gasification},2)}^{\text{out}} + w_{\text{H}_2\text{O}_{\text{waste}},(\text{Gasification},2)}^{\text{out}} + w_{\text{NH}_3,(\text{Gasification},2)}^{\text{out}} = y_{\text{Gasification}} \quad (\text{B.15})$$

$$w_{\text{SolidWaste},(\text{Gasification},3)}^{\text{out}} = y_{\text{Gasification}} \quad (\text{B.16})$$

The CAPEX for the gasification process is determined based on the total inlet mass flow using the following equation:

$$K_{\text{Gasification}}^{\text{cap}} = 13,300 \frac{\$}{\text{kg/h}} \cdot \dot{M}_{\text{Gasification}}^{\text{in,tot}}. \quad (\text{B.17})$$

### B.1.5. Autothermal reforming (ATR)

For the ATR process, we assume that a second outlet stream can be split from the product gas, which can be sent directly to the RWGS process to increase the CO content:

$$w_{\text{CH}_4,(\text{ATR},1)}^{\text{in}} + w_{\text{H}_2\text{O},(\text{ATR},1)}^{\text{in}} + w_{\text{O}_2,(\text{ATR},1)}^{\text{in}} = y_{\text{ATR}}, \quad (\text{B.18})$$

$$w_{\text{H}_2,(\text{ATR},1)}^{\text{out}} + w_{\text{CO},(\text{ATR},1)}^{\text{out}} + w_{\text{CO}_2,(\text{ATR},1)}^{\text{out}} + w_{\text{H}_2\text{O}_{\text{waste}},(\text{ATR},1)}^{\text{out}} = y_{\text{ATR}}, \quad (\text{B.19})$$

$$w_{\text{H}_2,(\text{ATR},2)}^{\text{out}} + w_{\text{CO}_2,(\text{ATR},2)}^{\text{out}} = y_{\text{ATR}}. \quad (\text{B.20})$$

Due to the unavailability of reliable cost scaling data for the AGR process as a function of process scale, its CAPEX is instead determined based on the total mass flow at the process inlet

$$K_{\text{AGR}}^{\text{cap}} = 243.5 \frac{\$}{\text{kg/h}} \cdot \dot{M}_{\text{AGR}}^{\text{in,tot}}, \quad (\text{B.21})$$

with the cost coefficient derived from the techno-economic data reported by Onel et al. [21].

### B.1.6. Electrolysis

$$w_{\text{H}_2\text{O},(j,1)}^{\text{in}} = y_j, \quad \forall j \in \{\text{AEC, PEMEC, SOEC}\} \quad (\text{B.22})$$

$$w_{\text{H}_2,(j,1)}^{\text{out}} = y_j, \quad \forall j \in \{\text{AEC, PEMEC, SOEC}\} \quad (\text{B.23})$$

$$w_{\text{O}_2,(j,2)}^{\text{out}} = y_j, \quad \forall j \in \{\text{AEC, PEMEC, SOEC}\} \quad (\text{B.24})$$

### B.1.7. Reverse water-gas shift (RWGS)

$$w_{\text{H}_2,(\text{RWGS},1)}^{\text{in}} + w_{\text{CO}_2,(\text{RWGS},1)}^{\text{in}} = y_{\text{RWGS}} \quad (\text{B.25})$$

$$w_{\text{H}_2,(\text{RWGS},1)}^{\text{out}} + w_{\text{CO}_2,(\text{RWGS},1)}^{\text{out}} + w_{\text{CO},(\text{RWGS},1)}^{\text{out}} + w_{\text{H}_2\text{O}_{\text{waste}},(\text{RWGS},1)}^{\text{out}} = y_{\text{RWGS}} \quad (\text{B.26})$$

$$w_{\text{H}_2\text{O}_{\text{waste}},(\text{RWGS},2)}^{\text{out}} = y_{\text{RWGS}} \quad (\text{B.27})$$

The CAPEX for the RWGS process is determined based on the total inlet mass flow using the following equation:

$$K_{\text{RWGS}}^{\text{cap}} = 2,070 \frac{\$}{\text{kg/h}} \cdot \dot{M}_{\text{RWGS}}^{\text{in,tot}}. \quad (\text{B.28})$$

### B.1.8. Acid gas removal (AGR)

Based on Liu et al. [5] we assume a  $\text{CO}_2$  capture rate of 62 % (mass-based) for the AGR process. This means that a pure  $\text{CO}_2$  outlet stream exits the AGR process via the second outlet port (modelled via Eq. B.31 and Eq. B.32), which can be fed directly to the CS process and sequestered. The remaining  $\text{CO}_2$  leaves the system with the other impurities via the boundaries as a sink flow.

$$w_{\text{H}_2,(\text{AGR},1)}^{\text{in}} + w_{\text{CO},(\text{AGR},1)}^{\text{in}} + w_{\text{CO}_2,(\text{AGR},1)}^{\text{in}} + w_{\text{H}_2\text{S},(\text{AGR},1)}^{\text{in}} + w_{\text{H}_2\text{O}_{\text{waste}},(\text{AGR},1)}^{\text{in}} + w_{\text{N}_2,(\text{AGR},1)}^{\text{in}} + w_{\text{HCl},(\text{AGR},1)}^{\text{in}} + w_{\text{CH}_4,(\text{AGR},1)}^{\text{in}} = y_{\text{AGR}} \quad (\text{B.29})$$

$$w_{\text{H}_2,(\text{AGR},1)}^{\text{out}} + w_{\text{CO},(\text{AGR},1)}^{\text{out}} = y_{\text{AGR}} \quad (\text{B.30})$$

$$w_{\text{CO}_2,(\text{AGR},2)}^{\text{out}} = y_{\text{AGR}} \quad (\text{B.31})$$

$$w_{\text{CO}_2,(\text{AGR},2)}^{\text{out}} \dot{M}_{\text{AGR},2}^{\text{out}} = 0.62 \cdot w_{\text{CO}_2,\text{AGR}}^{\text{in,tot}} \dot{M}_{\text{AGR}}^{\text{in,tot}} \quad (\text{B.32})$$

$$w_{\text{H}_2\text{S},(\text{AGR},3)}^{\text{out}} + w_{\text{CO}_2,(\text{AGR},3)}^{\text{out}} + w_{\text{N}_2,(\text{AGR},3)}^{\text{out}} + w_{\text{HCl},(\text{AGR},3)}^{\text{out}} + w_{\text{CH}_4,(\text{AGR},3)}^{\text{out}} + w_{\text{H}_2\text{O}_{\text{waste}},(\text{AGR},3)}^{\text{out}} = y_{\text{AGR}} \quad (\text{B.33})$$

### B.1.9. Fischer-Tropsch (FT)

$$w_{\text{H}_2,(\text{FT},1)}^{\text{in}} + w_{\text{CO},(\text{FT},1)}^{\text{in}} = y_{\text{FT}} \quad (\text{B.34})$$

$$\sum_{\alpha \in \mathcal{C}^{\text{HC}}} w_{\alpha,(\text{FT},1)}^{\text{out}} + w_{\text{H}_2\text{O}_{\text{waste}},(\text{FT},1)}^{\text{out}} = y_{\text{FT}} \quad (\text{B.35})$$

$$w_{\text{H}_2,(\text{FT},2)}^{\text{out}} + w_{\text{CO},(\text{FT},2)}^{\text{out}} = y_{\text{FT}} \quad (\text{B.36})$$

$$w_{\text{H}_2\text{O}_{\text{waste}},(\text{FT},3)}^{\text{out}} = y_{\text{FT}} \quad (\text{B.37})$$

The CAPEX for the FT process is determined based on the total inlet mass flow using the following equation:

$$K_{\text{FT}}^{\text{cap}} = 183 \frac{\$}{\text{kg/h}} \cdot \dot{M}_{\text{FT}}^{\text{in,tot}}. \quad (\text{B.38})$$

## C. Process flowsheet simulations

### C.1. Biomass gasification

The gasification process is simulated for three different types of biomass: miscanthus (MIS), wheat straw (WS), and pine chips (PC). The three types of biomass are characterized by different compositions, as shown in Tab. C.1.

Table C.1.: Proximate and ultimate analysis of different biomass types [17] used for the gasification ANN.

| biomass type | proximate analysis<br>(wt.%, dry) |      |      |     | ultimate analysis<br>(wt.%, dry) |          |        |        |         |         |
|--------------|-----------------------------------|------|------|-----|----------------------------------|----------|--------|--------|---------|---------|
|              | moisture                          | VM   | FC   | ash | C                                | O        | H      | N      | S       | Cl      |
| miscanthus   | 11.4                              | 81.2 | 15.8 | 3.0 | 47.724                           | 42.7964  | 5.82   | 0.388  | 0.1455  | 0.1261  |
| wheat straw  | 10.1                              | 74.8 | 18.1 | 7.1 | 45.8926                          | 39.96558 | 5.6669 | 0.6503 | 0.15793 | 0.56669 |
| pine chips   | 7.6                               | 72.4 | 21.6 | 6.0 | 49.632                           | 38.023   | 5.734  | 0.47   | 0.0846  | 0.0564  |

### C.2. Fischer-Tropsch (FT)

The chain growth probability and the resulting Anderson-Schulz-Flory (ASF) distribution are modeled as a function of reaction pressure, temperature and gas phase composition using an empirical FT reactor model.

In order to establish a relatively simple relationship between the product composition (for the sake of simplicity, we only consider n-alkanes as products) and the reaction conditions for cobalt-catalyzed FT synthesis, we apply an empirical model based on Hamelinck et al. [22]. This model considers product selectivity as a function of the  $H_2/CO$  ratio in the syngas, reaction pressure  $p_{FT}$ , and reaction temperature  $T_{FT}$  [22]. These parameters are linked to the selectivity of products with five and more carbon atoms  $S_{C_{5+}}$  via the following linear equation:

$$S_{C_{5+}} = 1.7 - 0.0024 \cdot T_{FT} - 0.088 \cdot \frac{[H_2]}{[CO]} + 0.18 \cdot ([H_2] + [CO]) + 0.0078 \cdot p_{FT}, \quad (C.1)$$

where  $[H_2]$  and  $[CO]$  represent the mole fractions of the two components in the feed gas. The impact of the parameters is evident in this equation. As indicated by the negative sign, an increase in  $H_2$  content and temperature results in a decrease in  $S_{C_{5+}}$ , which is

equivalent to the product distribution shifting towards lighter products and an increased methane production. Conversely, an increase in pressure and CO content leads to an increase in heavier products.

The chain growth probability  $\alpha$  can be connected to the selectivity  $S_{C_{5+}}$  using the following correlation [22]:

$$\alpha \approx 0.75 - 0.373 \cdot \sqrt{-\log(S_{C_{5+}})} + 0.25 \cdot S_{C_{5+}}. \quad (C.2)$$

The mole fractions  $x_n$  or mass fractions  $w_n$  for all hydrocarbons in the range from five to 30 carbon atoms are then determined by the ASF distribution:

$$x_n = (1 - \alpha) \alpha^{(n-1)}, \quad (C.3)$$

$$w_n = \alpha^{(n-1)} (1 - \alpha)^2 n, \quad (C.4)$$

where  $n$  denotes the number of carbon atoms. For hydrocarbons with a chain length of one to four carbon atoms, methane and ethane in particular, empirical measurements deviate from the ASF distribution. While methane formation is often underestimated by the ASF approach,  $C_2$  selectivity is usually overestimated [23]. In order to take this into account, the mass fractions of methane and the  $C_2$  to  $C_4$  hydrocarbons are not calculated according to Eq. C.4. Instead, the selectivity with regard to the short chain products is determined via:

$$S_{C_{1-4}} = 1 - S_{C_{5+}}. \quad (C.5)$$

The actual mass fractions are then calculated following de Klerk and adjusted to the selectivity  $S_{C_{1-4}}$  resulting from the process conditions [23]. The reference values for the mass fractions of the  $C_1$  to  $C_4$  components are provided in Tab. C.2.

Table C.2.: Reference mass fractions for the calculation of the FT reactor outlet mass fractions of the  $C_1$  to  $C_4$  components [23].

| component   | reference mass fraction / wt% |
|-------------|-------------------------------|
| $CH_4$      | 5.6                           |
| $C_2H_6$    | 1.1                           |
| $C_3H_8$    | 2.067                         |
| $C_4H_{10}$ | 3.133                         |

The sum of the reference mass fractions of the  $C_1$  to  $C_4$  products (0.119 in this case) is

divided by  $S_{C_{1-4}}$  to obtain a correction factor:

$$CF = \frac{0.119}{S_{C_{1-4}}}. \quad (C.6)$$

This correction factor is then multiplied with the reference mass fractions, resulting in the actual mass fractions of the  $C_1$  to  $C_4$  n-alkanes in the reactor outlet.

The original model also includes olefins. They are linked to the n-alkanes by an olefin/paraffin factor. Since only n-alkanes are considered in this work for reasons of simplification and the fraction of olefins in the total product mass is small, the olefins and thus the olefin-paraffin ratio are neglected. The mass fractions of the olefins are simply attributed to the corresponding n-alkanes with the same chain length.

Using the empirical approach described above, the mass fractions of all  $C_1$  to  $C_{30}$  n-alkanes in the outlet of the FT reactor can be calculated as a function of the reaction conditions (gas phase composition, pressure, and temperature). The FT reactor is modeled as a stoichiometric reactor in Aspen Plus<sup>®</sup>, where all reaction equations of the  $C_1$  to  $C_{30}$  n-alkanes are taken into account [20]. An Excel-calculator block routine is used to determine the product composition based on the empirical model. Unlike mechanistic-kinetic models, the empirical model used in our work does not consider CO conversion as a function of reaction conditions. For this reason, single-pass CO conversion is set at 70 %, based on typical values for cobalt-catalyzed FT synthesis, regardless of reaction conditions [22]. By calculating the mass and mole fractions of the individual products the CO conversion can be allocated proportionally to all the FT synthesis reactions. As a result, the FT Reactor Aspen Plus<sup>®</sup> simulation not only provides the output composition, but also the heat of reaction released in the reactor. Fig. C.1 shows ASF distributions as output of the FT Aspen Plus<sup>®</sup> flowsheet simulation based on the empirical reactor model for three sets of reaction conditions.

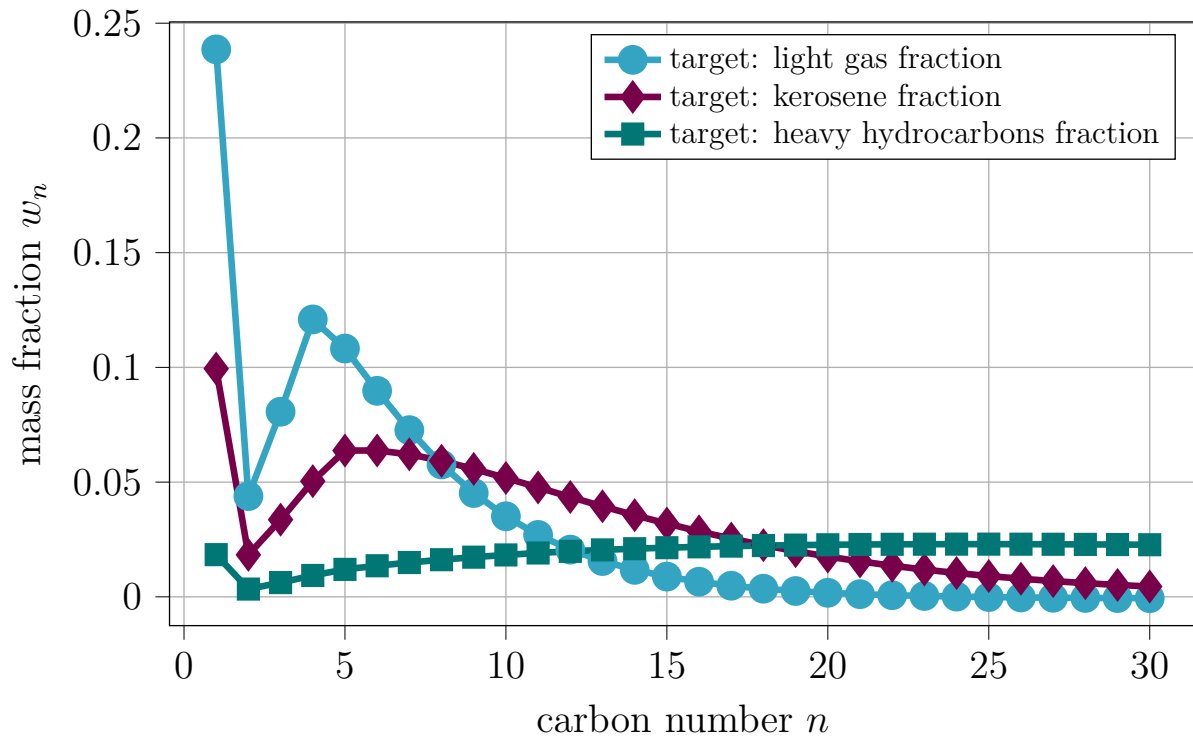

Figure C.1.: Corrected Anderson-Schulz-Flory (ASF) distribution for  $C_1$ - $C_{30}$  n-alkanes as output of the Fischer-Tropsch (FT) Aspen Plus<sup>®</sup> flowsheet simulation using the empirical FT reactor model. The reaction conditions used to target the light gas fraction are: molar  $H_2/CO = 2.28$ ,  $T_{FT} = 300\text{ }^\circ\text{C}$ ,  $p_{FT} = 30\text{ bar}$ . The reaction conditions used to target the kerosene fraction are: molar  $H_2/CO = 1.86$ ,  $T_{FT} = 230\text{ }^\circ\text{C}$ ,  $p_{FT} = 38\text{ bar}$ . The reaction conditions used to target the heavy hydrocarbons fraction are: molar  $H_2/CO = 1.82$ ,  $T_{FT} = 200\text{ }^\circ\text{C}$ ,  $p_{FT} = 50\text{ bar}$ .

## D. Artificial neural networks

### D.1. Outputs

#### D.1.1. Gasification

Outputs of the biomass gasification ANN:

- mass flow SCR-GAS/BIOMASS inflow
- $\text{H}_2$  mass fraction SCR-GAS out
- $\text{CO}$  mass fraction SCR-GAS out
- $\text{CO}_2$  mass fraction SCR-GAS out
- $\text{H}_2\text{O}$  mass fraction SCR-GAS out
- $\text{N}_2$  mass fraction SCR-GAS out
- $\text{HCl}$  mass fraction SCR-GAS out
- $\text{H}_2\text{S}$  mass fraction SCR-GAS out
- mass flow SOUR-H $2\text{O}$ /BIOMASS inflow
- $\text{CO}_2$  mass fraction SOUR-H $2\text{O}$  out
- $\text{H}_2\text{O}$  mass fraction SOUR-H $2\text{O}$  out
- mass flow LP-WATER/BIOMASS inflow
- net work PUMP-H $2\text{O}$ /BIOMASS inflow
- net heating duty HEAT-GAS/BIOMASS inflow
- net heating duty HEAT-H $2\text{O}$ /BIOMASS inflow
- net cooling duty GASIFIER/BIOMASS inflow
- net cooling duty COOL-SG/BIOMASS inflow

#### D.1.2. Reverse water-gas shift (RWGS)

Outputs of the RWGS ANN:

- mass flow SG-RWGS/TOTAL-IN inflow
- $\text{H}_2$  mass fraction SG-RWGS out
- $\text{CO}_2$  mass fraction SG-RWGS out
- $\text{CO}$  mass fraction SG-RWGS out
- net work C-RWGS/TOTAL-IN inflow
- net heating duty HWT-RWGS/TOTAL-IN inflow
- net heating duty RE-RWGS/TOTAL-IN inflow
- net cooling duty CWT-RWGS/TOTAL-IN inflow

#### D.1.3. Fischer-Tropsch (FT)

Outputs of the FT ANN:

- mass flow FT-C/SYNG-IN inflow
- $\text{H}_2\text{O}$  mass fraction FT-C out
- $\text{C}_n\text{H}_{2n+2}$   $\forall n = 1, \dots, 30$  mass fractions FT-C out
- mass flow FT-PURGE/SYNG-IN inflow
- $\text{H}_2$  mass fraction FT-PURGE out
- net work MS-COMP/SYNG-IN inflow
- net cooling duty MS-COMP/SYNG-IN inflow
- net cooling duty FT-REACT/SYNG-IN inflow
- net cooling duty FT-COOL/SYNG-IN inflow

## D.2. Hyperparameters

Table D.1.: Hyperparameters of best performing gasification, RWGS, and FT ANNs.

| hyperparameter                      | gasification       | RWGS               | FT                 |
|-------------------------------------|--------------------|--------------------|--------------------|
| # hidden ReLU layers                | 1                  | 1                  | 1                  |
| # input neurons                     | 7                  | 2                  | 3                  |
| # hidden ReLU neurons               | 75                 | 25                 | 100                |
| # output neurons*                   | 17                 | 8                  | 38                 |
| $\ell^1$ regularization coefficient | $1 \times 10^{-5}$ | $1 \times 10^{-4}$ | $1 \times 10^{-4}$ |
| initial learning rate**             | $1 \times 10^{-4}$ | $1 \times 10^{-4}$ | $1 \times 10^{-4}$ |
| maximum learning rate**             | $1 \times 10^{-2}$ | $1 \times 10^{-2}$ | $1 \times 10^{-2}$ |
| batch size                          | 40                 | 15                 | 5                  |
| epochs                              | 1000               | 1000               | 1000               |

\*Linear activation function is used for all the output neurons.

\*\*A cyclic learning rate, implemented in the Python package Keras, is used for ANN training [24]. The step size, which determines the duration of a single cycle for the cyclic learning rate, is determined by doubling the number of training data points and dividing it by the batch size.

### D.3. Parity plots

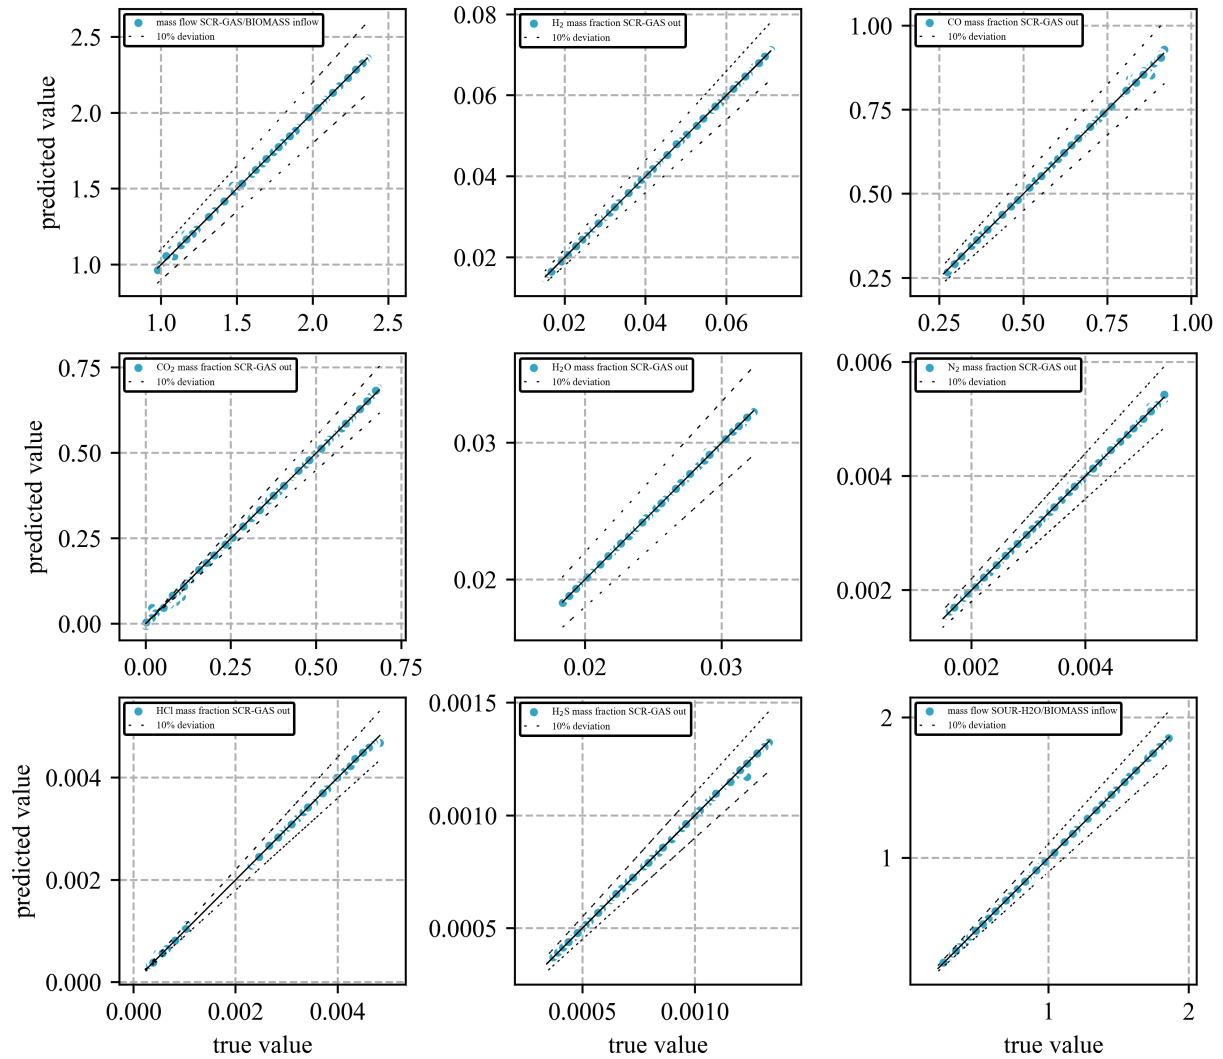

Figure D.1.: Parity plots of the biomass gasification artificial neural network. Test data points are shown for the first nine neural network outputs.

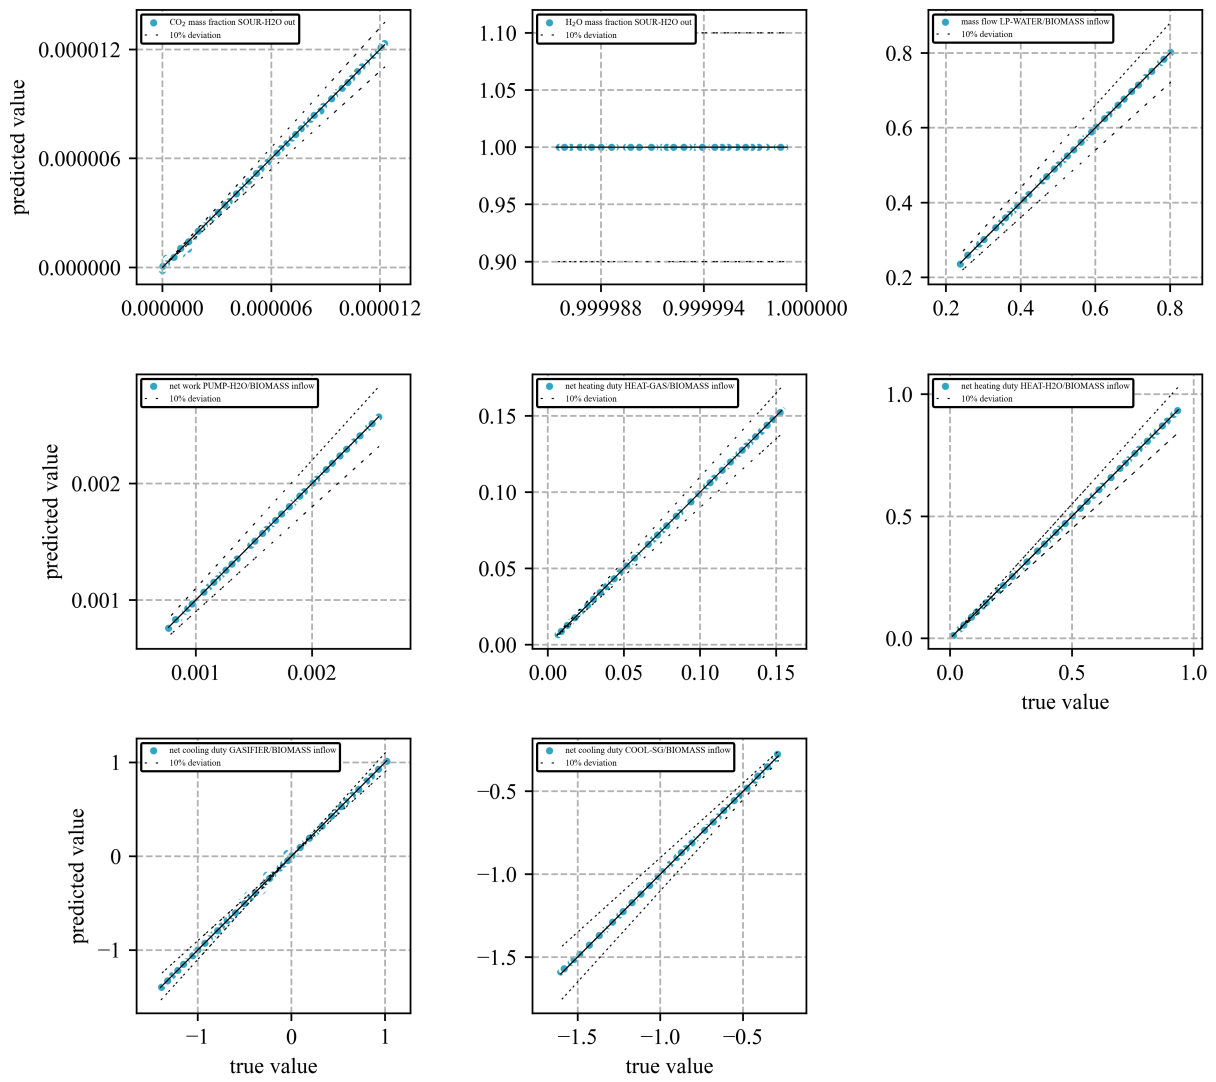

Figure D.2.: Parity plots of the biomass gasification artificial neural network. Test data points are shown for the last eight neural network outputs.

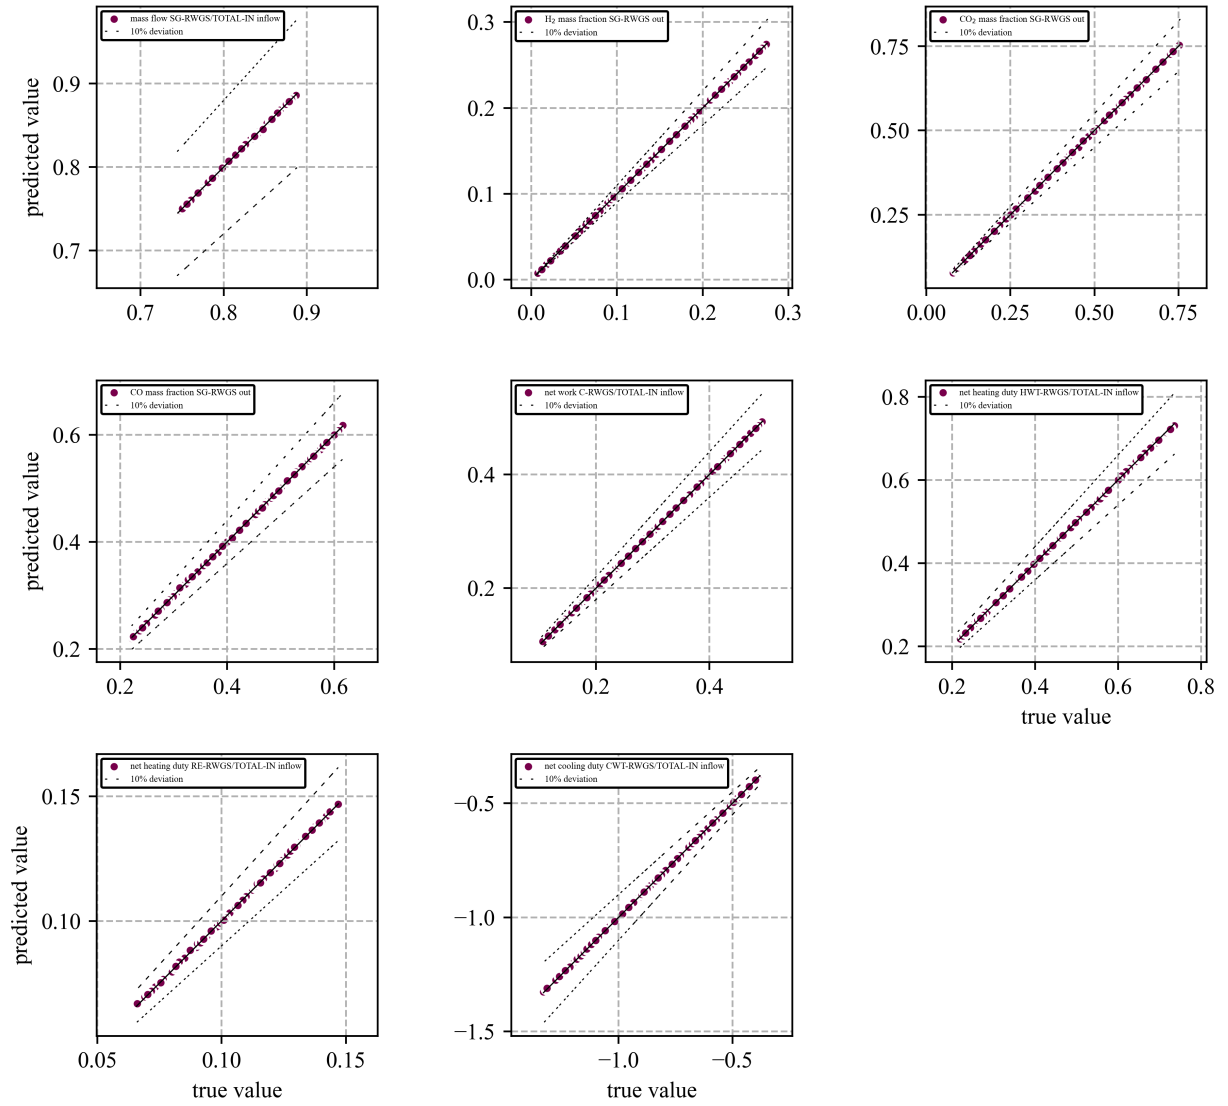

Figure D.3.: Parity plots of the reverse water-gas shift artificial neural network. Test data points are shown for all neural network outputs.

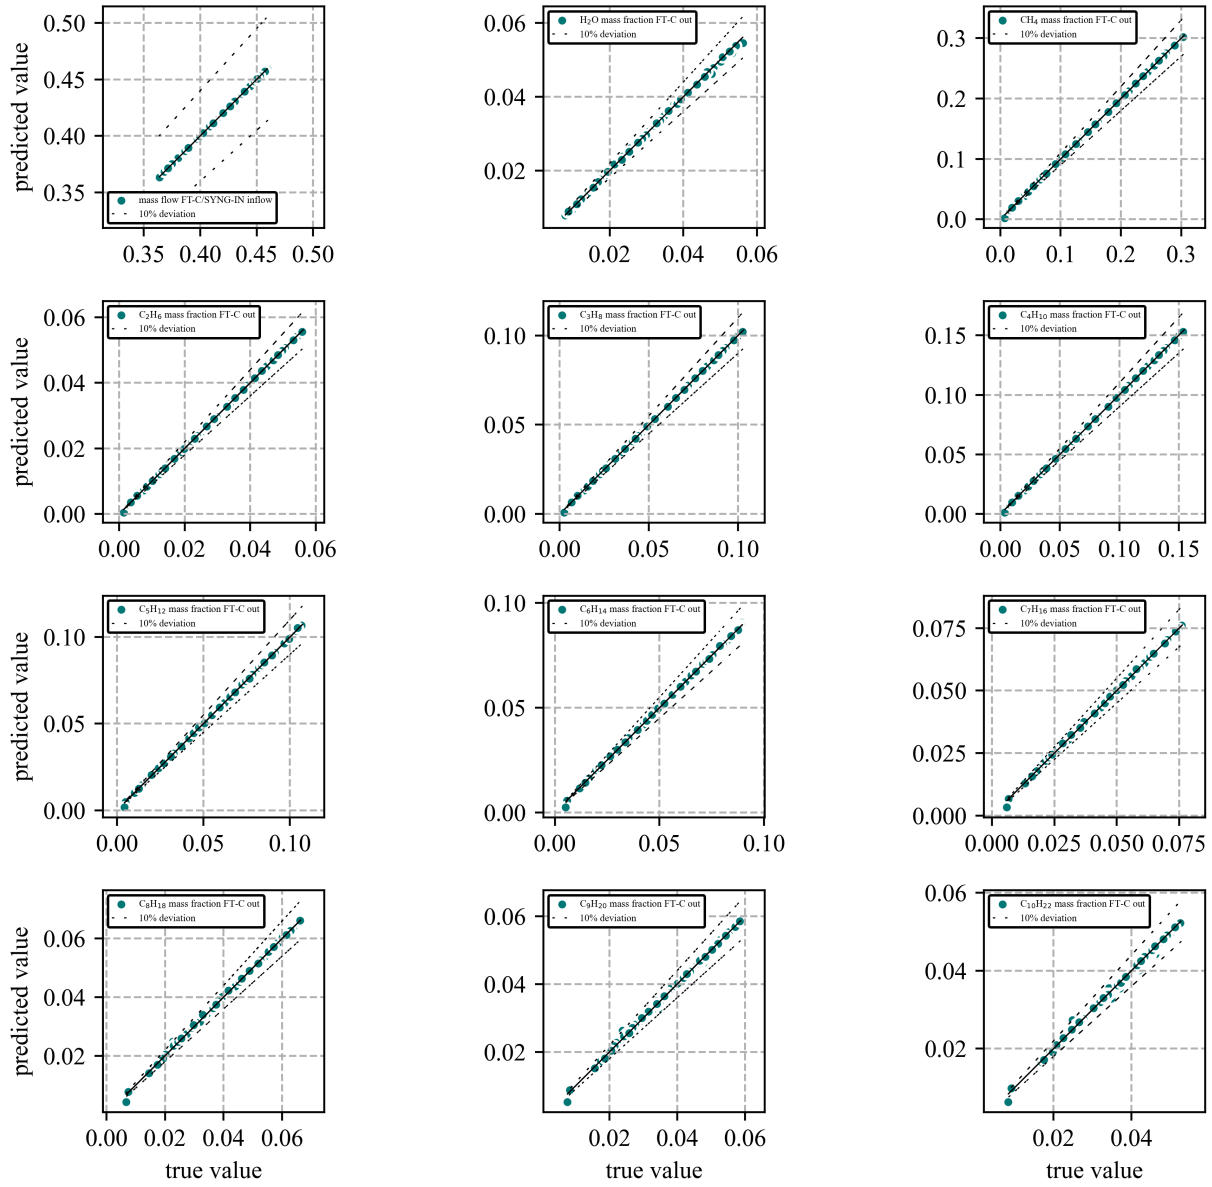

Figure D.4.: Parity plots of the Fischer-Tropsch artificial neural network. Test data points are shown for the first twelve neural network outputs.

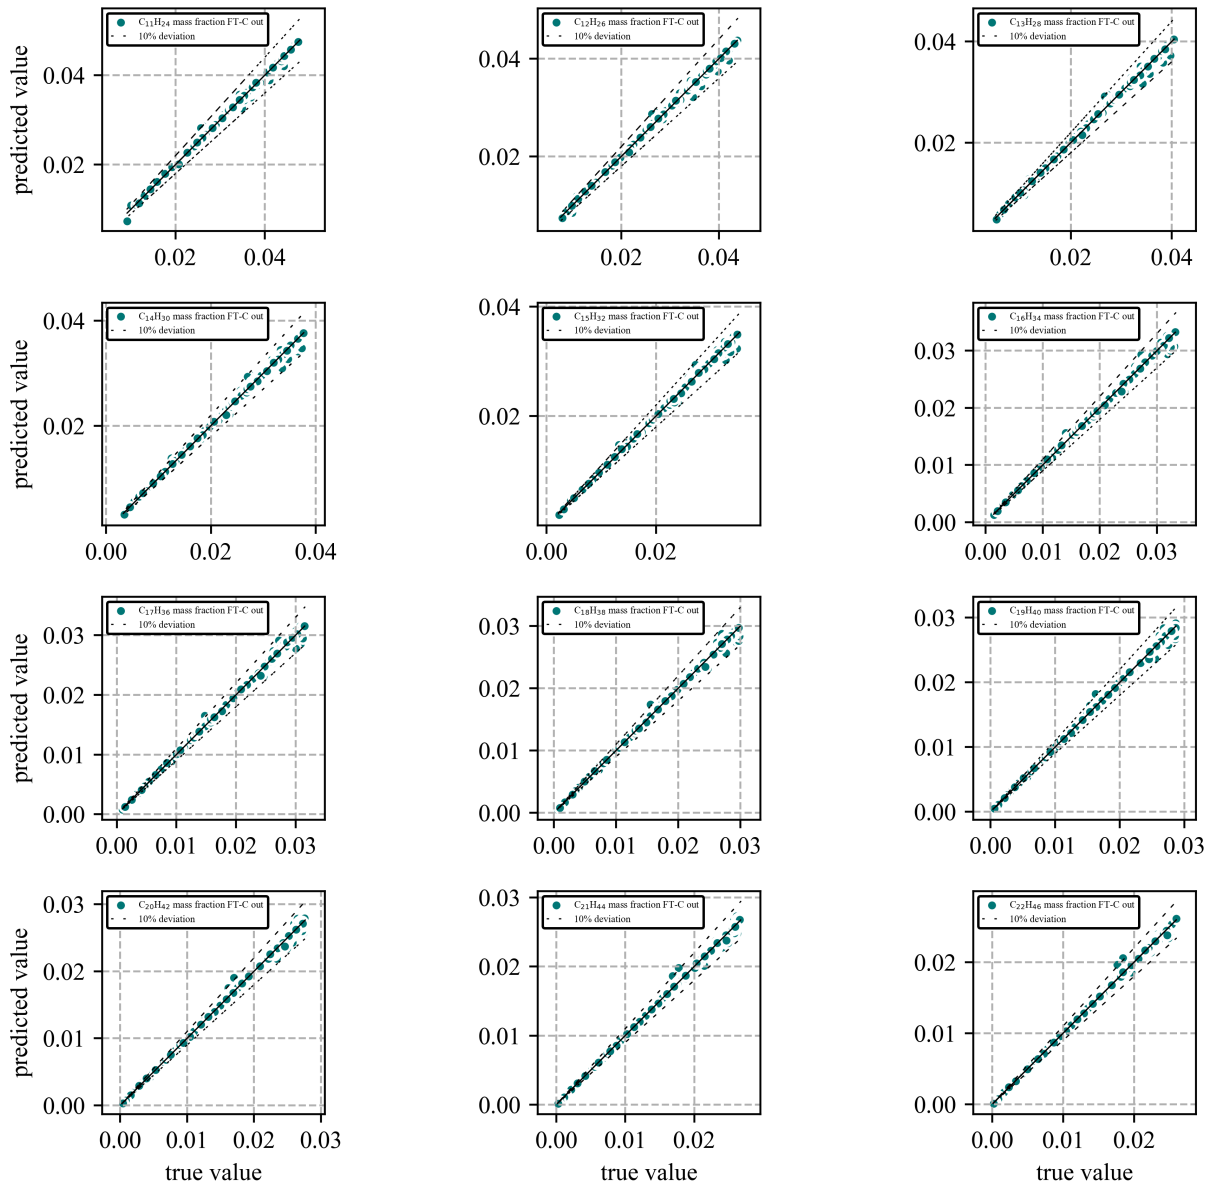

Figure D.5.: Parity plots of the Fischer-Tropsch artificial neural network. Test data points are shown for outputs 13-24.

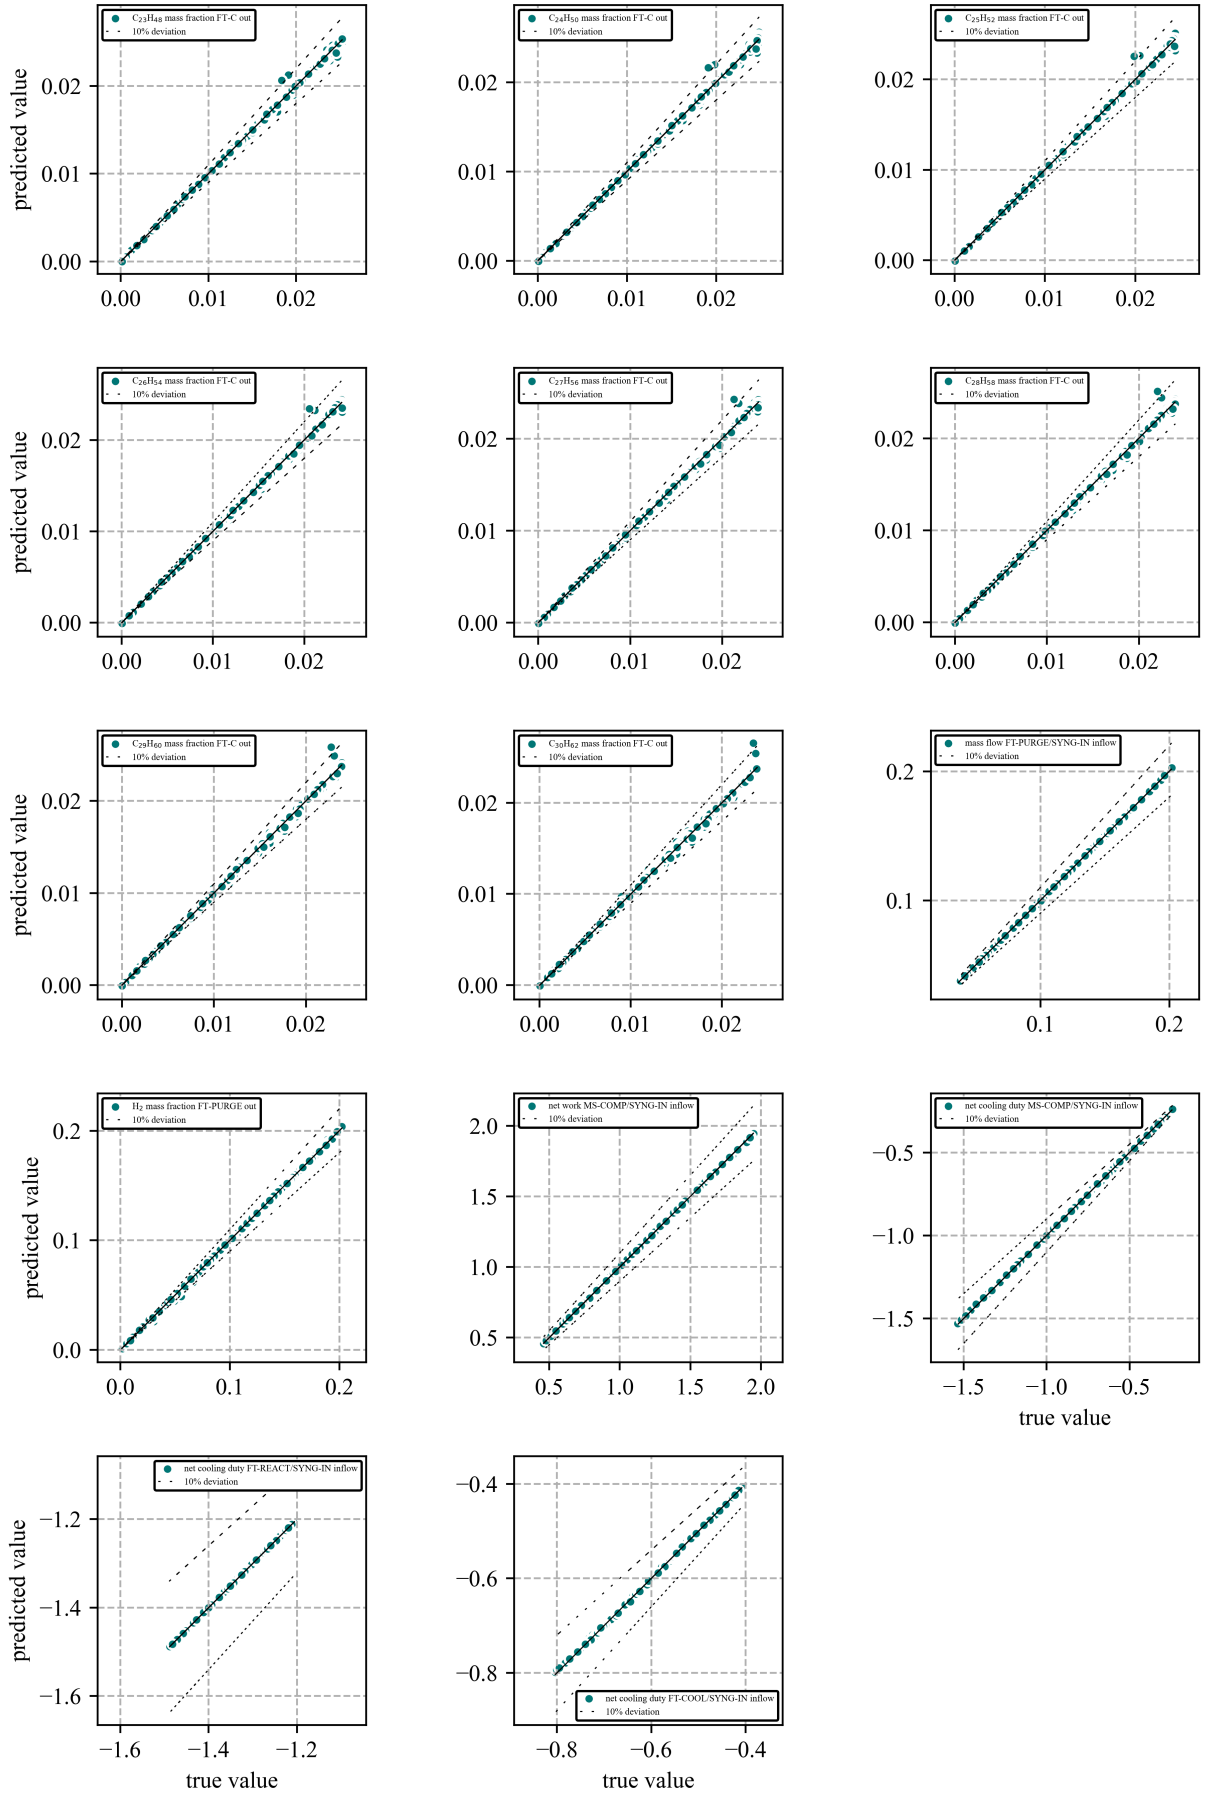

Figure D.6.: Parity plots of the Fischer-Tropsch artificial neural network. Test data points are shown for outputs 25-38.

## D.4. Embedding of artificial neural networks in the superstructure optimization framework

To embed the trained ANNs in the MIQCP superstructure optimization, the decision variables describing the ANN inputs and outputs (denoted by  $f_{j,(\text{input},i)}^{\text{ANN}}$  and  $f_{j,(\text{output},o)}^{\text{ANN}}$  for process  $j$  and input/output  $i/o$ ) are linked to the decision variables in the superstructure via equality constraints. All of these equality constraints for embedding the ANNs for the gasification, RWGS and FT process are listed below. Since not all ANN outputs are dependent on the mass flow entering the flowsheets (e.g., component mass fractions within outlet streams), the inlet mass flow is not used as input for the ANNs in order to avoid numerical problems during optimization. Instead, the inlet mass flow is optimized as a decision variable of the MIQCP formulation. The ANN outputs depending on this mass flow (e.g., work and heat requirements) are determined by ratios with respect to this inlet mass flow (see also outputs of the trained ANNs based on the Aspen Plus<sup>®</sup> flowsheet simulations in Section D.1).

### D.4.1. Gasification

$$x_{\text{Miscanthus}} = f_{\text{Gasification},(\text{input},1)}^{\text{ANN}}, \quad (\text{D.1})$$

$$x_{\text{WheatStraw}} = f_{\text{Gasification},(\text{input},2)}^{\text{ANN}}, \quad (\text{D.2})$$

$$x_{\text{PineChips}} = f_{\text{Gasification},(\text{input},3)}^{\text{ANN}}, \quad (\text{D.3})$$

$$\dot{M}_{(\text{Gasification},2)}^{\text{in}} = f_{\text{Gasification},(\text{input},4)}^{\text{ANN}} \dot{M}_{(\text{Gasification},1)}^{\text{in}}, \quad (\text{D.4})$$

$$\dot{M}_{(\text{Gasification},3)}^{\text{in}} = f_{\text{Gasification},(\text{input},5)}^{\text{ANN}} \dot{M}_{(\text{Gasification},1)}^{\text{in}}, \quad (\text{D.5})$$

$$\dot{M}_{(\text{Gasification},4)}^{\text{in}} = f_{\text{Gasification},(\text{input},6)}^{\text{ANN}} \dot{M}_{(\text{Gasification},1)}^{\text{in}}, \quad (\text{D.6})$$

$$T_{(\text{Gasification},2)} = f_{\text{Gasification},(\text{input},7)}^{\text{ANN}}, \quad (\text{D.7})$$

$$\dot{M}_{(\text{Gasification},1)}^{\text{out}} = f_{\text{Gasification},(\text{output},1)}^{\text{ANN}} \dot{M}_{(\text{Gasification},1)}^{\text{in}}, \quad (\text{D.8})$$

$$w_{\text{H}_2,(\text{Gasification},1)}^{\text{out}} = y_{\text{Gasification}} f_{\text{Gasification},(\text{output},2)}^{\text{ANN}}, \quad (\text{D.9})$$

$$w_{\text{CO},(\text{Gasification},1)}^{\text{out}} = y_{\text{Gasification}} f_{\text{Gasification},(\text{output},3)}^{\text{ANN}}, \quad (\text{D.10})$$

$$w_{\text{CO}_2,(\text{Gasification},1)}^{\text{out}} = y_{\text{Gasification}} f_{\text{Gasification},(\text{output},4)}^{\text{ANN}}, \quad (\text{D.11})$$

$$w_{\text{H}_2\text{O}_{\text{waste}},(\text{Gasification},1)}^{\text{out}} = y_{\text{Gasification}} f_{\text{Gasification},(\text{output},5)}^{\text{ANN}}, \quad (\text{D.12})$$

$$w_{\text{N}_2,(\text{Gasification},1)}^{\text{out}} = y_{\text{Gasification}} f_{\text{Gasification},(\text{output},6)}^{\text{ANN}}, \quad (\text{D.13})$$

$$w_{\text{HCl},(\text{Gasification},1)}^{\text{out}} = y_{\text{Gasification}} f_{\text{Gasification},(\text{output},7)}^{\text{ANN}}, \quad (\text{D.14})$$

$$w_{\text{H}_2\text{S},(\text{Gasification},1)}^{\text{out}} = y_{\text{Gasification}} f_{\text{Gasification},(\text{output},8)}^{\text{ANN}}, \quad (\text{D.15})$$

$$\dot{M}_{(\text{Gasification},2)}^{\text{out}} = f_{\text{Gasification},(\text{output},9)}^{\text{ANN}} \dot{M}_{(\text{Gasification},1)}^{\text{in}}, \quad (\text{D.16})$$

$$w_{\text{CO}_2,(\text{Gasification},2)}^{\text{out}} = y_{\text{Gasification}} f_{\text{Gasification},(\text{output},10)}^{\text{ANN}}, \quad (\text{D.17})$$

$$w_{\text{H}_2\text{O}_{\text{waste}},(\text{Gasification},2)}^{\text{out}} = y_{\text{Gasification}} f_{\text{Gasification},(\text{output},11)}^{\text{ANN}}, \quad (\text{D.18})$$

$$\dot{M}_{(\text{Gasification},5)}^{\text{in}} = f_{\text{Gasification},(\text{output},12)}^{\text{ANN}} \dot{M}_{(\text{Gasification},1)}^{\text{in}}, \quad (\text{D.19})$$

$$\dot{W}_{\text{Gasification}} = f_{\text{Gasification},(\text{output},13)}^{\text{ANN}} \dot{M}_{(\text{Gasification},1)}^{\text{in}}, \quad (\text{D.20})$$

$$\dot{W}_{\text{Gasification}} \leq 0 \quad (\text{D.21})$$

The heat demand required for the first heat integration port of the gasification process is comprised of the heat demand for heating the gasification agents to 450 °C and the heat demand for the biomass decomposition step. The ratio of the heat requirement for the decomposition step to the biomass inlet flow is approximately constant, other heat requirements are calculated according to the gasification ANN:

$$\begin{aligned} \dot{Q}_{(\text{Gasification},1)} = & \left( f_{\text{Gasification},(\text{output},14)}^{\text{ANN}} + f_{\text{Gasification},(\text{output},15)}^{\text{ANN}} \right. \\ & \left. - 1.552 \right) \dot{M}_{(\text{Gasification},1)}^{\text{in}}, \end{aligned} \quad (\text{D.22})$$

$$\dot{Q}_{(\text{Gasification},2)} = f_{\text{Gasification},(\text{output},16)}^{\text{ANN}} \dot{M}_{(\text{Gasification},1)}^{\text{in}}, \quad (\text{D.23})$$

$$\dot{Q}_{(\text{Gasification},3)} = f_{\text{Gasification},(\text{output},17)}^{\text{ANN}} \dot{M}_{(\text{Gasification},1)}^{\text{in}}. \quad (\text{D.24})$$

#### D.4.2. Reverse water-gas shift (RWGS)

$$T_{(\text{RWGS},1)} = f_{\text{RWGS},(\text{input},1)}^{\text{ANN}}, \quad (\text{D.25})$$

$$w_{\text{H}_2,(\text{RWGS},1)}^{\text{in}} = y_{\text{RWGS}} f_{\text{RWGS},(\text{input},2)}^{\text{ANN}}, \quad (\text{D.26})$$

$$\dot{M}_{(\text{RWGS},1)}^{\text{out}} = f_{\text{RWGS},(\text{output},1)}^{\text{ANN}} \dot{M}_{(\text{RWGS},1)}^{\text{in}}, \quad (\text{D.27})$$

$$w_{\text{H}_2,(\text{RWGS},1)}^{\text{out}} = y_{\text{RWGS}} f_{\text{RWGS},(\text{output},2)}^{\text{ANN}}, \quad (\text{D.28})$$

$$w_{\text{CO}_2,(\text{RWGS},1)}^{\text{out}} = y_{\text{RWGS}} f_{\text{RWGS},(\text{output},3)}^{\text{ANN}}, \quad (\text{D.29})$$

$$w_{\text{CO},(\text{RWGS},1)}^{\text{out}} = y_{\text{RWGS}} f_{\text{RWGS},(\text{output},4)}^{\text{ANN}}, \quad (\text{D.30})$$

$$\dot{W}_{\text{RWGS}} = f_{\text{RWGS},(\text{output},5)}^{\text{ANN}} \dot{M}_{(\text{RWGS},1)}^{\text{in}}, \quad (\text{D.31})$$

$$\dot{W}_{\text{RWGS}} \leq 0, \quad (\text{D.32})$$

$$\dot{Q}_{(\text{RWGS},1)} = \left( f_{\text{RWGS},(\text{output},6)}^{\text{ANN}} + f_{\text{RWGS},(\text{output},7)}^{\text{ANN}} \right) \dot{M}_{(\text{RWGS},1)}^{\text{in}}, \quad (\text{D.33})$$

$$\dot{Q}_{(\text{RWGS},2)} = f_{\text{RWGS},(\text{output},8)}^{\text{ANN}} \dot{M}_{(\text{RWGS},1)}^{\text{in}} \quad (\text{D.34})$$

#### D.4.3. Fischer-Tropsch (FT)

$$T_{(\text{FT},1)} = f_{\text{FT},(\text{input},1)}^{\text{ANN}}, \quad (\text{D.35})$$

$$p_{\text{FT}} = f_{\text{FT},(\text{input},2)}^{\text{ANN}}, \quad (\text{D.36})$$

$$w_{\text{H}_2,(\text{FT},1)}^{\text{in}} = y_{\text{FT}} f_{\text{FT},(\text{input},3)}^{\text{ANN}}, \quad (\text{D.37})$$

$$\dot{M}_{(\text{FT},1)}^{\text{out}} = f_{\text{FT},(\text{output},1)}^{\text{ANN}} \dot{M}_{(\text{FT},1)}^{\text{in}}, \quad (\text{D.38})$$

$$w_{\text{H}_2\text{O}_{\text{waste}},(\text{FT},1)}^{\text{out}} = y_{\text{FT}} f_{\text{FT},(\text{output},2)}^{\text{ANN}}, \quad (\text{D.39})$$

$$w_{\text{C}_n\text{H}_{2n+2},(\text{FT},1)}^{\text{out}} = y_{\text{FT}} f_{\text{FT},(\text{output},n+2)}^{\text{ANN}} \quad \forall n = 1, \dots, 30, \quad (\text{D.40})$$

$$\dot{M}_{(\text{FT},2)}^{\text{out}} = f_{\text{FT},(\text{output},33)}^{\text{ANN}} \dot{M}_{(\text{FT},1)}^{\text{in}}, \quad (\text{D.41})$$

$$w_{\text{H}_2,(\text{FT},2)}^{\text{out}} = y_{\text{FT}} f_{\text{FT},(\text{output},34)}^{\text{ANN}}, \quad (\text{D.42})$$

$$\dot{W}_{\text{FT}} = f_{\text{FT},(\text{output},35)}^{\text{ANN}} \dot{M}_{(\text{FT},1)}^{\text{in}}, \quad (\text{D.43})$$

$$\dot{W}_{\text{FT}} \leq 0, \quad (\text{D.44})$$

$$\dot{Q}_{(\text{FT},1)} = \left( f_{\text{FT},(\text{output},36)}^{\text{ANN}} + f_{\text{FT},(\text{output},37)}^{\text{ANN}} \right) \dot{M}_{(\text{FT},1)}^{\text{in}}, \quad (\text{D.45})$$

$$\dot{Q}_{(\text{FT},2)} = f_{\text{FT},(\text{output},38)}^{\text{ANN}} \dot{M}_{(\text{FT},1)}^{\text{in}} \quad (\text{D.46})$$

## E. Results

### E.1. CO<sub>2</sub> abatement costs

Table E.1.: CO<sub>2</sub> abatement costs, specific CO<sub>2</sub> emissions, and specific cost for Pareto optimal designs on the curve for specific kerosene costs vs. CO<sub>2</sub> emissions (Fig. 7). Counting starts from the right of the Pareto curve (the first point corresponds to the design with the lowest costs and highest CO<sub>2</sub> emissions and the sixth point belongs to the design with the highest costs and lowest CO<sub>2</sub> emissions). CO<sub>2</sub> abatement costs are always calculated in relation to our fossil ATR reference design.

| design number | CO <sub>2</sub> abatement costs /<br>\$/t <sub>CO<sub>2</sub></sub> | specific CO <sub>2</sub> emissions /<br>kg <sub>CO<sub>2</sub></sub> /kg <sub>kerosene</sub> | specific cost /<br>\$/kg <sub>kerosene</sub> |
|---------------|---------------------------------------------------------------------|----------------------------------------------------------------------------------------------|----------------------------------------------|
| 1             | -                                                                   | 4.47                                                                                         | 0.79                                         |
| 2             | 211                                                                 | 3.14                                                                                         | 1.07                                         |
| 3             | 246                                                                 | 1.76                                                                                         | 1.46                                         |
| 4             | 379                                                                 | 0.27                                                                                         | 2.38                                         |
| 5             | 440                                                                 | -0.98                                                                                        | 3.18                                         |
| 6             | 486                                                                 | -2.22                                                                                        | 4.04                                         |

Table E.2.: Specific CO<sub>2</sub> emissions, specific cost, and CO<sub>2</sub> abatement costs for various cases with regard to carbon sequestration, CO<sub>2</sub> footprints, and GHG emission targets. CO<sub>2</sub> abatement costs are always calculated in relation to our fossil ATR reference design. Results are generated excluding the fossil ATR process.

| case | sequestration<br>permitted | supply chain<br>emissions biomass | CO <sub>2</sub> emissions<br>electricity and heat | net zero<br>target | specific CO <sub>2</sub><br>emissions /<br>kgCO <sub>2</sub> /kgkerosene | specific<br>cost /<br>\$/kgkerosene | CO <sub>2</sub> abatement<br>costs /<br>\$/tCO <sub>2</sub> |
|------|----------------------------|-----------------------------------|---------------------------------------------------|--------------------|--------------------------------------------------------------------------|-------------------------------------|-------------------------------------------------------------|
| 1    | ✓                          | ✓                                 | ✓                                                 | ✗                  | 3.74                                                                     | 1.82                                | 1,408.68                                                    |
| 2    | ✓                          | ✓                                 | ✓                                                 | ✓                  | 0                                                                        | 2.58                                | 399.04                                                      |
| 3    | ✓                          | ✓                                 | ✗                                                 | ✗                  | 1.54                                                                     | 1.82                                | 350.86                                                      |
| 4    | ✓                          | ✓                                 | ✗                                                 | ✓                  | 0                                                                        | 1.95                                | 258.03                                                      |
| 5    | ✓                          | ✗                                 | ✓                                                 | ✗                  | 2.29                                                                     | 1.82                                | 472.23                                                      |
| 6    | ✓                          | ✗                                 | ✓                                                 | ✓                  | 0                                                                        | 2.09                                | 290.92                                                      |
| 7    | ✓                          | ✗                                 | ✗                                                 | ✗                  | 0                                                                        | 1.82                                | 234.87                                                      |
| 8    | ✓                          | ✗                                 | ✗                                                 | ✓                  | 0                                                                        | 1.82                                | 234.87                                                      |
| 9    | ✗                          | ✓                                 | ✓                                                 | ✗                  | 3.74                                                                     | 1.82                                | 1,408.68                                                    |
| 10   | ✗                          | ✓                                 | ✓                                                 | ✓                  | infeasible                                                               |                                     |                                                             |
| 11   | ✗                          | ✗                                 | ✓                                                 | ✗                  | 2.29                                                                     | 1.82                                | 472.23                                                      |
| 12   | ✗                          | ✗                                 | ✓                                                 | ✓                  | infeasible                                                               |                                     |                                                             |
| 13   | ✗                          | ✓                                 | ✗                                                 | ✗                  | 1.54                                                                     | 1.82                                | 350.86                                                      |
| 14   | ✗                          | ✓                                 | ✗                                                 | ✓                  | 0                                                                        | 4.49                                | 844.74                                                      |
| 15   | ✗                          | ✗                                 | ✗                                                 | ✗                  | 0                                                                        | 1.82                                | 234.87                                                      |
| 16   | ✗                          | ✗                                 | ✗                                                 | ✓                  | 0                                                                        | 1.82                                | 234.87                                                      |

## E.2. Pareto-optimal solutions

### E.2.1. Cost vs. biomass usage

Fig. E.1 shows the Pareto curve and the corresponding C and H sources for specific kerosene cost vs. biomass usage, excluding the fossil ATR process and without any restrictions on  $\text{CO}_2$  emissions. The specific cost ranges from 1.82  $\$/\text{kg}_{\text{kerosene}}$  (no restrictions on biomass) to 3.52  $\$/\text{kg}_{\text{kerosene}}$  (no use of biomass permitted). With increasing restrictions on the amount of biomass, C from point sources and H from electrolysis are used.

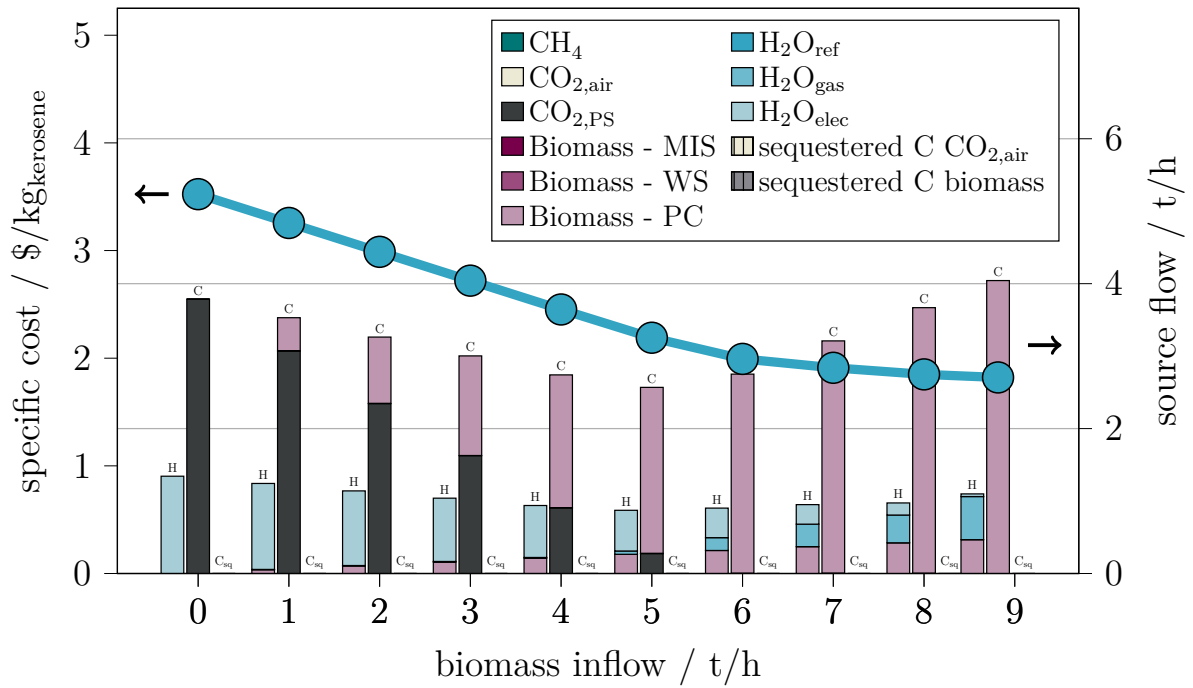

Figure E.1.: Pareto-optimal designs for specific kerosene cost vs. biomass usage (left y-axis). The bars represent the source flows for carbon (C) and hydrogen (H) entering the system (right y-axis). The third bar shows sequestered carbon ( $\text{C}_{\text{sq}}$ ) either from  $\text{CO}_2$  from the air or from biomass. Results are generated **excluding the fossil autothermal reforming (ATR) process and without any restrictions on  $\text{CO}_2$  emissions**. (PS: point source; MIS: miscanthus; WS: wheat straw; PC: pine chips; ref: reforming; gas: gasification; elec: electrolysis).

Fig. E.2 shows the Pareto curve and the corresponding C and H sources for specific kerosene cost vs. biomass usage, excluding the fossil ATR process, external  $\text{CO}_2$  from point sources, and without any restrictions on  $\text{CO}_2$  emissions. Compared to Fig. E.1, C is now provided via DAC with increasing restrictions on biomass use. The specific cost ranges from 1.82  $\$/\text{kg}_{\text{kerosene}}$  (no restrictions on biomass) to 4.14  $\$/\text{kg}_{\text{kerosene}}$  (no use of biomass permitted). The higher costs arise due to the fact that  $\text{CO}_2$  from DAC is more expensive than  $\text{CO}_2$  from point sources.

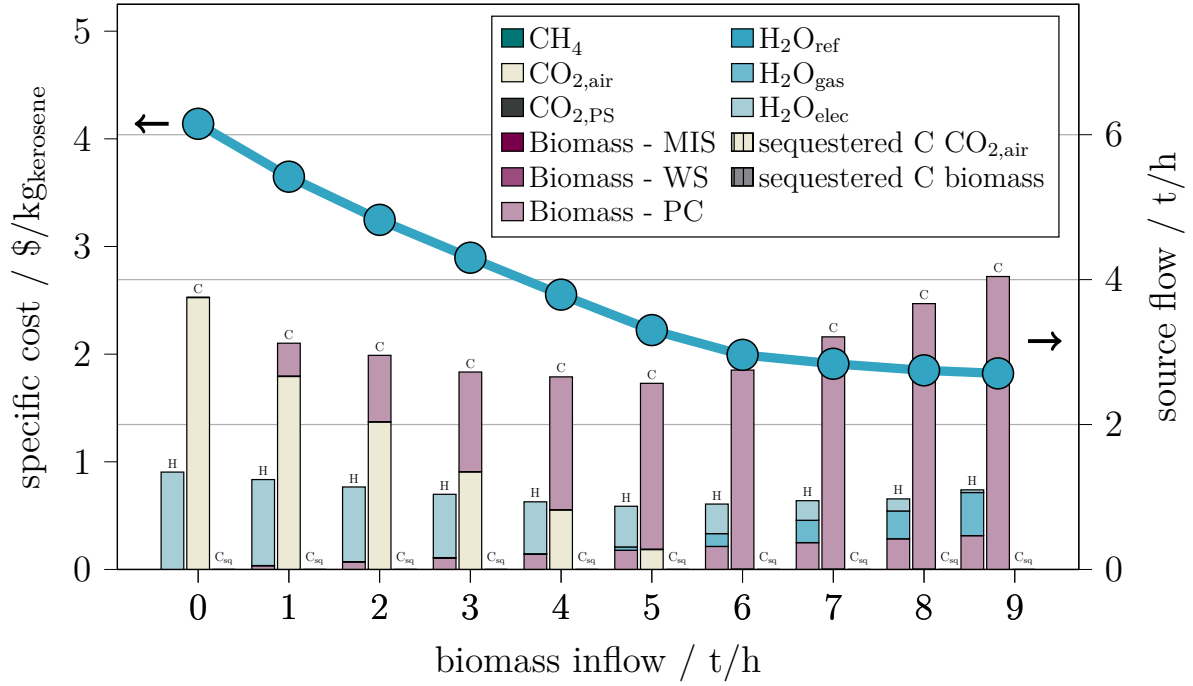

Figure E.2.: Pareto-optimal designs for specific kerosene cost vs. biomass usage (left y-axis). The bars represent the source flows for carbon (C) and hydrogen (H) entering the system (right y-axis). The third bar shows sequestered carbon ( $C_{\text{sq}}$ ) either from  $\text{CO}_2$  from the air or from biomass. Results are generated **excluding the fossil autothermal reforming (ATR) process, external  $\text{CO}_2$  from point sources, and without any restrictions on  $\text{CO}_2$  emissions.** (PS: point source; MIS: miscanthus; WS: wheat straw; PC: pine chips; ref: reforming; gas: gasification; elec: electrolysis).

Fig. E.3 shows the Pareto curve and the corresponding C and H sources for specific kerosene cost vs. biomass usage, excluding the fossil ATR process. Additionally,  $\text{CO}_2$  emissions are set to  $0 \text{ kg}_{\text{CO}_2}/\text{kg}_{\text{kerosene}}$ . The specific cost ranges from  $2.58 \text{ \$/kg}_{\text{kerosene}}$  (no restrictions on biomass) to  $11 \text{ \$/kg}_{\text{kerosene}}$  (no use of biomass permitted). This cost increase is driven by the additional need for carbon sequestration (due to the high  $\text{CO}_2$  emissions associated with the provision of electricity for water electrolysis) to achieve the net-zero target.

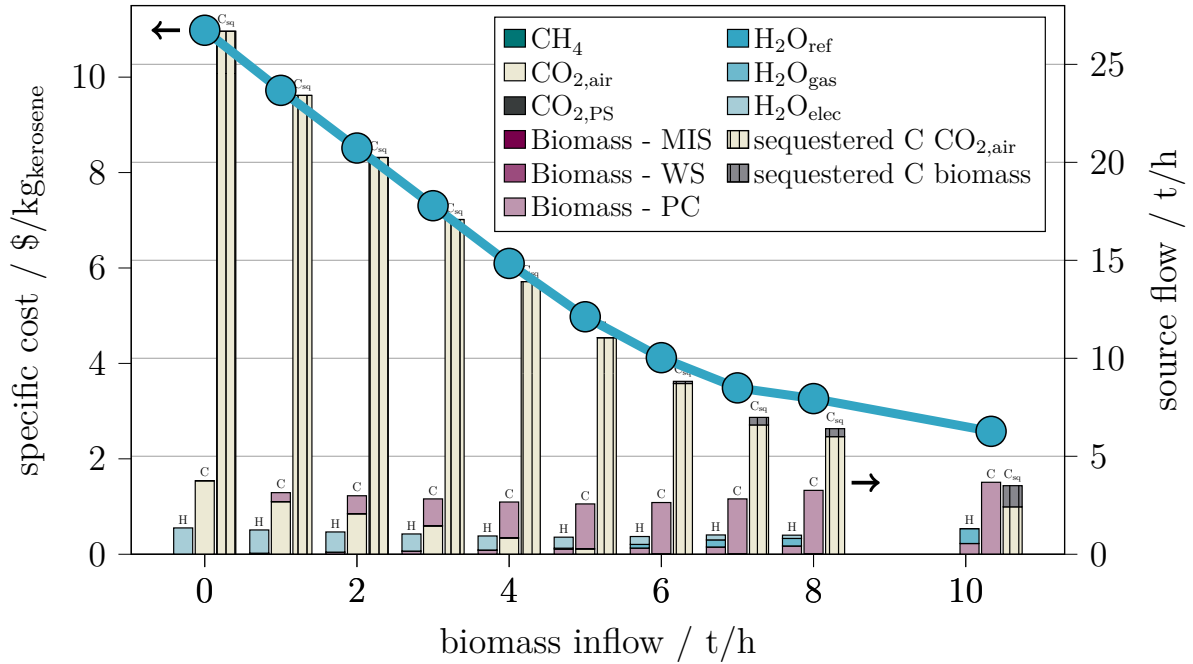

Figure E.3.: Pareto-optimal designs for specific kerosene cost vs. biomass usage (left y-axis). The bars represent the source flows for carbon (C) and hydrogen (H) entering the system (right y-axis). The third bar shows sequestered carbon ( $C_{\text{sq}}$ ) either from  $\text{CO}_2$  from the air or from biomass. Results are generated **excluding the fossil autothermal reforming (ATR) process**.  $\text{CO}_2$  emissions are set to  $0 \text{ kg}_{\text{CO}_2}/\text{kg}_{\text{kerosene}}$ . (PS: point source; MIS: miscanthus; WS: wheat straw; PC: pine chips; ref: reforming; gas: gasification; elec: electrolysis).

### E.2.2. Cost vs. CO<sub>2</sub> emissions

Fig. E.4 shows the Pareto curve and the corresponding C and H sources for specific kerosene cost vs. specific CO<sub>2</sub> emissions, excluding the fossil ATR and the gasification process. The specific cost ranges from 3.52 \$/kg<sub>kerosene</sub> (no restrictions on CO<sub>2</sub> emissions) to 12.5 \$/kg<sub>kerosene</sub> (−2.22 kgCO<sub>2</sub>/kg<sub>kerosene</sub>). In all cases, H is produced by electrolysis, while C is initially obtained from point sources and enters the system via DAC as emissions are increasingly restricted. Due to the high electricity requirements of electrolysis, the heat requirements of DAC, and the associated CO<sub>2</sub> footprints, it is necessary to sequester a large amount of C from the air in order to achieve the emission targets. This leads to a drastic rise in specific cost for carbon negative kerosene compared to the biomass-based route.

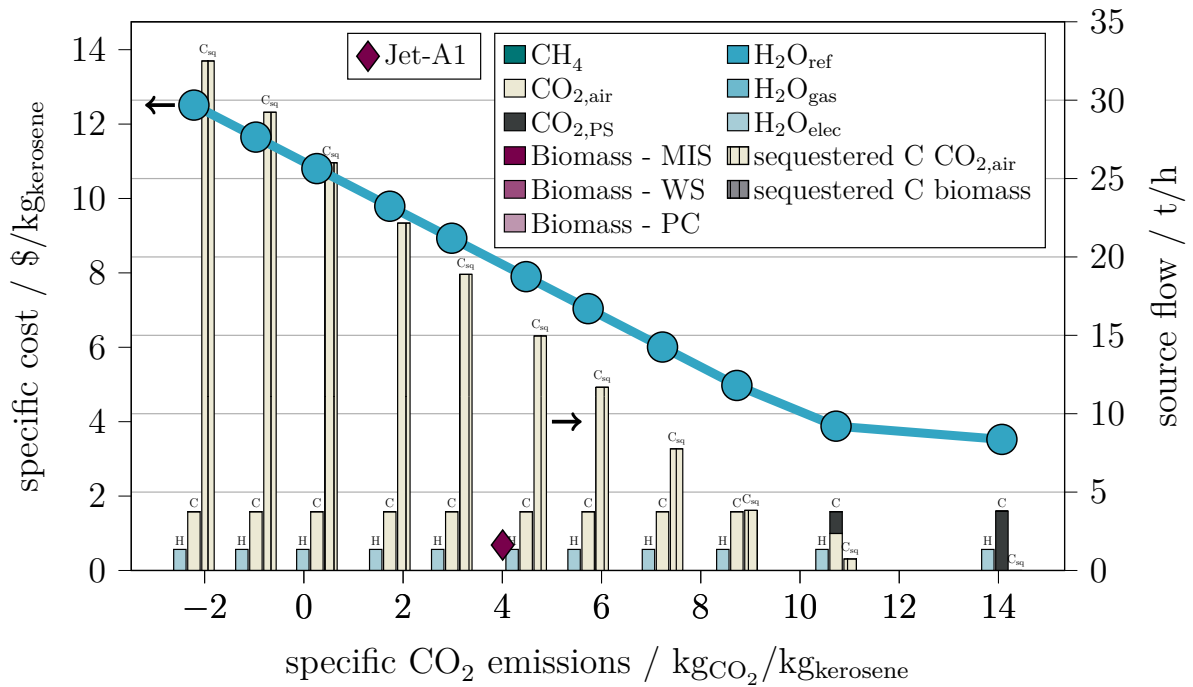

Figure E.4.: Pareto-optimal designs for specific kerosene cost vs. specific CO<sub>2</sub> emissions (left y-axis). The bars represent the source flows for carbon (C) and hydrogen (H) entering the system (right y-axis). The third bar shows sequestered carbon (C<sub>sq</sub>) either from CO<sub>2</sub> from the air or from biomass. Results are generated **excluding the fossil autothermal reforming (ATR) process and the gasification process**. (PS: point source; MIS: miscanthus; WS: wheat straw; PC: pine chips; ref: reforming; gas: gasification; elec: electrolysis).

Fig. E.5 shows the Pareto curve and the corresponding C and H sources for specific kerosene cost vs. specific CO<sub>2</sub> emissions, excluding the fossil ATR and the gasification process. Furthermore, CO<sub>2</sub> emissions related to the provision of electricity and heat are set to 0 kg<sub>CO<sub>2</sub>-eq</sub>/kWh. The specific cost range from 3.52 \$/kg<sub>kerosene</sub> (no restrictions on CO<sub>2</sub> emissions) to 4.46 \$/kg<sub>kerosene</sub> (−2.22 kg<sub>CO<sub>2</sub></sub>/kg<sub>kerosene</sub>). The sources for C and H are in any case the same as in Fig. E.4. However, the cost curve is significantly flatter, as the CO<sub>2</sub> footprints of electricity and heat are neglected, reducing the amount of C that needs to be sequestered to achieve the emission targets.

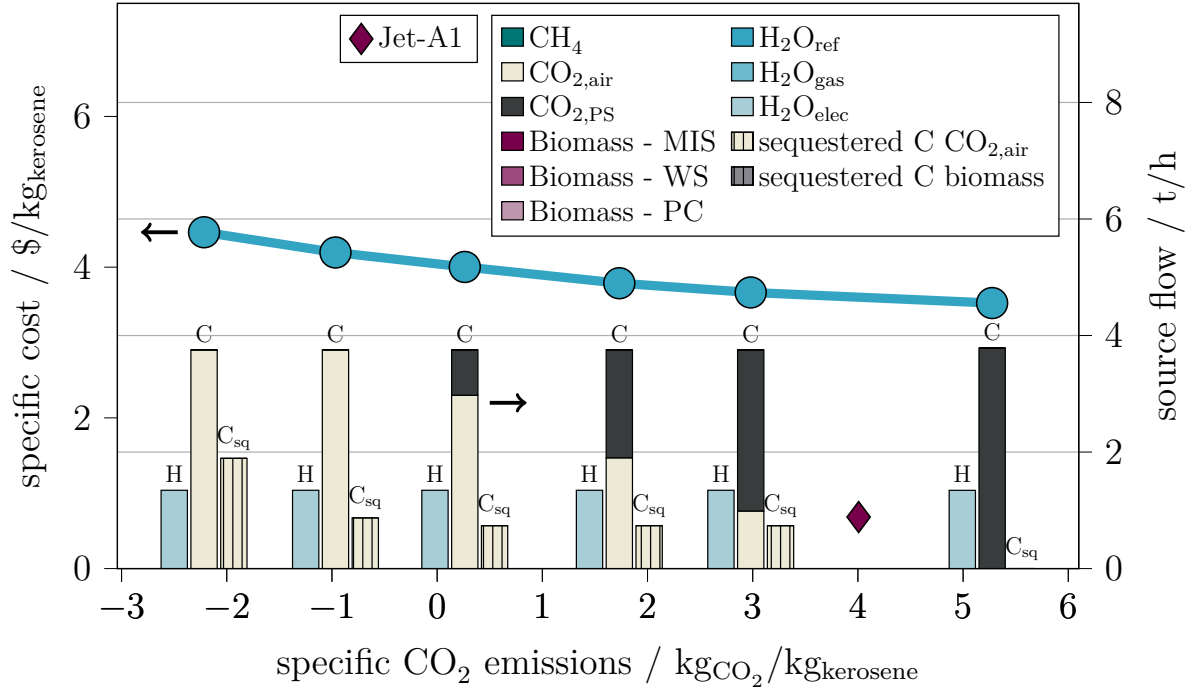

Figure E.5.: Pareto-optimal designs for specific kerosene cost vs. specific CO<sub>2</sub> emissions (left y-axis). The bars represent the source flows for carbon (C) and hydrogen (H) entering the system (right y-axis). The third bar shows sequestered carbon (C<sub>sq</sub>) either from CO<sub>2</sub> from the air or from biomass. Results are generated **excluding the fossil autothermal reforming (ATR) process and the gasification process. Furthermore, CO<sub>2</sub> emissions related to the provision of electricity and heat are set to 0 kg<sub>CO<sub>2</sub>-eq</sub>/kWh.** (PS: point source; MIS: miscanthus; WS: wheat straw; PC: pine chips; ref: reforming; gas: gasification; elec: electrolysis).

# References

- [1] T. Svitnič and K. Sundmacher. “Renewable methanol production: Optimization-based design, scheduling and waste-heat utilization with the FluxMax approach”. In: *Applied Energy* 326 (2022), p. 120017. ISSN: 0306-2619. DOI: 10.1016/j.apenergy.2022.120017.
- [2] C. D. Demirhan, W. W. Tso, J. B. Powell, and E. N. Pistikopoulos. “A multi-scale energy systems engineering approach towards integrated multi-product network optimization”. In: *Applied Energy* 281 (2021), p. 116020. ISSN: 0306-2619. DOI: 10.1016/j.apenergy.2020.116020.
- [3] M. J. Palys, I. Mitrai, and P. Daoutidis. “Renewable hydrogen and ammonia for combined heat and power systems in remote locations: Optimal design and scheduling”. In: *Optimal Control Applications and Methods* (2021), pp. 1–20. ISSN: 0143-2087. DOI: 10.1002/oca.2793.
- [4] A. O. Oni, K. Anaya, T. Giwa, G. Di Lullo, and A. Kumar. “Comparative assessment of blue hydrogen from steam methane reforming, autothermal reforming, and natural gas decomposition technologies for natural gas-producing regions”. In: *Energy Conversion and Management* 254 (2022), p. 115245. ISSN: 0196-8904. DOI: 10.1016/j.enconman.2022.115245.
- [5] X. Liu, S. Yang, Z. Hu, and Y. Qian. “Simulation and assessment of an integrated acid gas removal process with higher CO<sub>2</sub> capture rate”. In: *Computers & Chemical Engineering* 83 (2015), pp. 48–57. ISSN: 0098-1354. DOI: 10.1016/j.compchemeng.2015.01.008.
- [6] T. Svitnič, K. Beer, K. Sundmacher, and M. Böcher. “Optimal design of a sector-coupled renewable methanol production amid political goals and expected conflicts: Costs vs. land use”. In: *Sustainable Production and Consumption* 44 (2024), pp. 123–150. ISSN: 23525509. DOI: 10.1016/j.spc.2023.12.003.
- [7] A. Gonzalez-Garay, C. Heuberger-Austin, X. Fu, M. Klokkenburg, D. Zhang, A. van der Made, and N. Shah. “Unravelling the potential of sustainable aviation fuels to decarbonise the aviation sector”. In: *Energy & Environmental Science* 15.8 (2022), pp. 3291–3309. ISSN: 1754-5692. DOI: 10.1039/D1EE03437E.

- [8] P. Kenkel, T. Wassermann, and E. Zondervan. “Biogas Reforming as a Precursor for Integrated Algae Biorefineries: Simulation and Techno-Economic Analysis”. In: *Processes* 9.8 (2021), p. 1348. ISSN: 2227-9717. DOI: 10.3390/pr9081348.
- [9] J. Kim, J. Park, M. Qi, I. Lee, and I. Moon. “Process Integration of an Autothermal Reforming Hydrogen Production System with Cryogenic Air Separation and Carbon Dioxide Capture Using Liquefied Natural Gas Cold Energy”. In: *Industrial & Engineering Chemistry Research* 60.19 (2021), pp. 7257–7274. ISSN: 0888-5885. DOI: 10.1021/acs.iecr.0c06265.
- [10] D. Yang, P. Balaprakash, and S. Leyffer. “Modeling design and control problems involving neural network surrogates”. In: *Computational Optimization and Applications* 83.3 (2022), pp. 759–800. DOI: 10.1007/s10589-022-00404-9.
- [11] C. Ganzer and N. Mac Dowell. “A comparative assessment framework for sustainable production of fuels and chemicals explicitly accounting for intermittency”. In: *Sustainable Energy & Fuels* 4.8 (2020), pp. 3888–3903. ISSN: 2398-4902. DOI: 10.1039/C9SE01239G.
- [12] K. H. R. Rouwenhorst, P. M. Krzywda, N. E. Benes, G. Mul, and L. Lefferts. “Ammonia, 4. Green Ammonia Production”. In: *Ullmann’s Encyclopedia of Industrial Chemistry*. 7. edition, release 2015. Weinheim and Wiley online library: Wiley-VCH, 2010, pp. 1–20. ISBN: 3527306730. DOI: 10.1002/14356007.w02\_w02.
- [13] R. Meys, A. Kätelhön, M. Bachmann, B. Winter, C. Zibunas, S. Suh, and A. Bardow. “Achieving net-zero greenhouse gas emission plastics by a circular carbon economy”. In: *Science* 374.6563 (2021), pp. 71–76. DOI: 10.1126/science.abg9853.
- [14] D. Nebeská, J. Trögl, D. Žofková, A. Voslařová, J. Štojdl, and V. Pidlisnyuk. “Calorific values of Miscanthus x giganteus biomass cultivated under suboptimal conditions in marginal soils”. In: *Studia Oecologica* 13.1 (2020), pp. 61–67. ISSN: 1802-212X. DOI: 10.21062/ujep/429.2020/a/1802-212x/so/13/1/61.
- [15] Trading Economics. *EU Natural Gas TTF - Price - Chart - Historical Data - News*. 30.04.2025. URL: <https://tradingeconomics.com/commodity/eu-natural-gas>.
- [16] C. Cumicheo, N. Mac Dowell, and N. Shah. “Natural gas and BECCS: A comparative analysis of alternative configurations for negative emissions power generation”. In: *International Journal of Greenhouse Gas Control* 90 (2019), p. 102798. ISSN: 1750-5836. DOI: 10.1016/j.ijggc.2019.102798.
- [17] S. V. Vassilev, D. Baxter, L. K. Andersen, and C. G. Vassileva. “An overview of the chemical composition of biomass”. In: *Fuel* 89.5 (2010), pp. 913–933. ISSN: 0016-2361. DOI: 10.1016/j.fuel.2009.10.022.

- 
- [18] C. D. Demirhan, W. W. Tso, J. B. Powell, and E. N. Pistikopoulos. “Sustainable ammonia production through process synthesis and global optimization”. In: *AIChE Journal* 65.7 (2019), e16498. DOI: 10.1002/aic.16498.
- [19] S. Voß, S. Bube, and M. Kaltschmitt. “Hybrid Biomass- and Electricity-Based Kerosene Production-A Techno-Economic Analysis”. In: *Energy & Fuels* 38.6 (2024), pp. 5263–5278. ISSN: 0887-0624. DOI: 10.1021/acs.energyfuels.3c04876.
- [20] Aspen Technology Inc. *Aspen Plus*. 30.04.2024. URL: <https://www.aspentech.com/en/products/engineering/aspen-plus>.
- [21] O. Onel, A. M. Niziolek, J. A. Elia, R. C. Baliban, and C. A. Floudas. “Biomass and Natural Gas to Liquid Transportation Fuels and Olefins (BGTL+C2\_C4): Process Synthesis and Global Optimization”. In: *Industrial & Engineering Chemistry Research* 54.1 (2015), pp. 359–385. ISSN: 0888-5885. DOI: 10.1021/ie503979b.
- [22] C. Hamelinck, A. Faaij, H. den Uil, and H. Boerrigter. “Production of FT transportation fuels from biomass; technical options, process analysis and optimisation, and development potential”. In: *Energy* 29.11 (2004), pp. 1743–1771. ISSN: 0360-5442. DOI: 10.1016/j.energy.2004.01.002.
- [23] A. de Klerk. *Fischer–Tropsch Refining*. Wiley, 2011. ISBN: 9783527326051. DOI: 10.1002/9783527635603.
- [24] KerasTeam. *Keras: Deep Learning for humans*. 30.04.2025. URL: <https://keras.io/>.
